# Supplementary material for: Conditional Invertible Neural Networks for Diverse Image-to-Image Translation
Source: arXiv:2105.02104 source file (2021-05-05)
Supplement: Supplementary file 1 [file 05_WHOLE_APPENDIX.tex]

\newpage

\begin{center}
{\bf \Large 
Conditional Invertible Neural Networks \\ \noindent for Diverse Image-to-Image Translation \\[3mm] \noindent
-- Appendix --} \\[3mm] \noindent
Submission ID 70
\end{center}
\appendix
\section{Proofs and Assumptions}

\newcommand{\cn}{\varphi}
\newcommand{\Go}{\mathcal{G}_0}
\newcommand{\Gi}{\mathcal{G}_1}
\newcommand*{\QED}[1][$\square$]{%
\leavevmode\unskip\penalty9999 \hbox{}\nobreak\hfill
    \quad\hbox{#1}%
}

We further disambiguate the notation used in the main paper:
upper case letter (e.g. $X$) denote random variables (RVs),
and lower case letters denote their instances (e.g. $x$).
We write the probability distribution of a RV as $p(X)$,
and its evaluated density at any point $p(x)$, or $p(X=x)$ where ambiguous.
We include the INNs network parameters $\theta$ implicitly in $f$, and write
$f(\cdot; \hat \theta) \eqqcolon \hat f(\cdot)$, as well as
$q(x \mid c, \theta) \eqqcolon q(x \mid c)$ and 
$q(x \mid c, \hat \theta) \eqqcolon \hat q(x \mid c)$,
to simplify the equations.
We also write the loss as a functional depending on $f$ and $\cn$ for clarity:
$\cml = \cml[ f, \cn]$.
We also understand the argmin and argmax operations to return a set,
because the extremum must not necessarily be unique.
So, we write $\hat a \in \operatorname{arg\,min}\mathcal{L}(a)$ instead of `$=$' as in the main paper.
We also restate the propositions according to this notation.

We consider the RVs $X,Y$ jointly: $[X,Y] :\Omega \to (\mathcal{X}, \mu)$ 
with the measurable space $(\mathcal{X}, \mu)$ ,
where $\mathcal{X} = \mathcal{X}_X \times \mathcal{X}_Y = \mathbb{R}^{d_X + d_Y}$ 
is the domain of $x, y$,
and $\mu$ is the Lebesgue measure.
We assume $p(X,Y)$ is absolutely continuous w.r.t. $\mu$.
We make use of the differential entropy and differential conditional entropy $H$,
see \cite[Ch. 8.1]{cover2012elements} for definitions.

For the loss, we do not take a finite number of training samples into account,
and instead assume that the loss $\cml[f, \cn]$ is the exact expecation over the training data distribution $p(X,Y)$.
Strong consistency of the loss for the empirical expectation can be shown in the usual way,
assuming a compact parameter space and bounded outputs of the INN,
and applying Chebyshev's Inequality, but this is beyond the scope of this work,
and greatly complicates the form of the propositions.

To outline the proofs in the following section:
We first state and discuss some assumptions about the INN $f$ and the conditioning network $\cn$,
which are required in our proofs of the propositions.
Lemma 1 states two inequalities, which bound the loss from below.
Under Assumptions 1, 2 and 3, we show that choices of $f$ and $\cn$ exist 
where each bound is met exactly.
Lastly, for each proposition, we show that when the respective bound from Lemma 1 is met exactly,
the Proposition holds true.
\\[3mm]
\textbf{Assumption 1. }{\it
We assume that the INN is chosen from a family of distributional universal approximators $\mathcal{F}$,
as defined in \cite{teshima2020coupling}.
}
\\[3mm]
This simply means that the INN is in principle powerful enough to represent any distribution $p(X\mid C)$.
Affine coupling block INNs specifically were recently proven to satisfy this in \cite{teshima2020coupling},
under some requirements for the subnetworks.
Their result readily generalizes to CCBs, by changing the definition for $\mathcal{H}$ in Sec. D of \cite{teshima2020coupling}.
Proving this rigorously is beyond the scope of this work, 
so we leave the universality of the INN as an assumption.
\\[3mm]
\textbf{Assumption 2.}{\it
We assume that the conditioning network $\cn: \mathbb{R}^{d_Y} \to \mathbb{R}^{d_C}$
is chosen from the set $\Go$, which is defined as the set of all functions, 
for which the pushforward measure $p(C) \equiv p(\cn(Y)) \coloneqq \cn \sharp p(Y)$ is absolutely continuous w.r.t. the Lebesgue measure.
}
\\[3mm]
What this means intuitively, is that no subset of features can be exactly the same, 
or otherwise perfectly inter-dependent.
This is mostly a formal requirement: 
if it is not fulfilled, it does damage or alter the outcome of the training,
it simply means the MI is ill-defined, and Proposition 1 can not be formulated in the same way.
Proposition 2 can still be shown, by slightly altering Lemma 1 to avoid using the MI,
see e.g. \cite{beaudry2011intuitive} for an alternative formulation of the data processing inequality,
that applies even if the assumption does not hold.
\\[3mm]
\textbf{Assumption 3. }{\it
In addition to Assumption 2,
we assume that $\cn$ is chosen from $\Gi$, 
where $\Gi$ is a family of universal approximators as defined in \cite{hornik1989multilayer}.
Secondly, we assume the number of features extracted, $d_C \coloneqq \dim(C)$
is $\geq d_Y \coloneqq \dim(Y)$.
}\\[3mm]
This assumption is stronger than Assumption 2, and is a sufficient condition to show Proposition 2.
Intuitively, it says that $\cn$ must have sufficient expressive power so that the features $C$ 
can be informative enough for the INN to reproduce the true posterior.
This includes the number of features, and the network power.
If the features are too few, or inaccurate and uninformative, 
the INN will not be able to model the true posterior. \\[3mm]
\noindent
\textbf{Lemma 1. }{\it
Denoting the pushforward measure as $p(C) \equiv p(\cn(Y)) \coloneqq \cn \sharp p(Y)$,
the following inequality holds for all choices of $\cn$, $f$:
\begin{equation}
    \cml[f, \cn] 
    \underset{(a)}{\geq} H\big(X \mid \cn(Y)\big)
    \underset{(b)}{\geq} H\big(X \mid Y \big)
\end{equation}
Under Assumption 1, a choice of $f \in \mathcal{F}$ exists where (a) is equal, 
and under Assumption 3 a choice of $\cn \in \Gi$ exists where (b) becomes equal.
} \\[3mm] \noindent
\textbf{Proof. }{
    Because $\cml$ is equivalent to the definition of the differential cross-entropy $H_p(q(X\mid \cn(Y)))$,
    (a) follows directly from the inequality that the cross entropy is $\geq$ the entropy 
    with equality iff $p = q$ \cite[p. 256]{cover2012elements}.
    Assumption 1 guarantees that $f$ can be chosen so that $p(X\mid \cn(Y)) = q(X \mid \cn(Y))$,
    and therefore (a) becomes `='.

    (b) follows from the information processing inequality \cite[p. 34]{cover2012elements},
    whereby
    \begin{equation}
        I(X, Y) \geq I(X, \cn(Y)).
        \label{eq:data_processing}
    \end{equation}
    Writing out the terms, and subtracting the constant $H(X)$ from both sides directly yields (b).
    Therefore, (b) becomes `=' iff Eq. \ref{eq:data_processing} is also `='.
    We can construct a $\cn$ for which this is the case using Assumption 3 as a sufficient condition:
    We split up $C$ into $C = [C_s, C_n]$, where $\dim(C_s) = \dim(Y)$ and $\dim(C_n) = \dim(C) - \dim(Y) \geq 0$.
    According to \cite[Corollary 4.2]{hornik1989multilayer},
    we can choose $\cn$ such that that the mapping $\cn_s: Y \to C_s$ is a homeomorphism,
    and $C_n$ only contains constants (or noise), independent of $Y$. This part can effectively be ignored.
    Using this construction, we get
    \begin{equation}
        I(X, \cn(Y)) = I(X, \cn_s(Y)) = I(X, Y).
    \end{equation}
    We used the independence of $C_n$ and $Y$ in the first step, 
    and the invariance of the MI under homeomorphic transforms \cite[Eq. A2]{kraskov2004estimating}
    in the second step.
    \QED
}
\\[3mm]
\textbf{Proposition 1. }{\it
Let $\hat f$ be the INN and $\hat \cn$ the conditioning network that jointly minimize $\cml$,
where $\cn$ is optimized over $\Go$ given in Assumption 2, and $f$ over $\mathcal{F}$ given in Assumption 1.
Then it holds that
\begin{equation}
    I \big(X, \hat \cn(Y) \big) = \underset{\varphi \in \Go}{\operatorname {max}} \; I \big(X, \cn(Y) \big) 
\end{equation}
}
\\[3mm]
\textbf{Proof.}
Recall the minimization process
\begin{equation}
    \hat f, \hat \cn \in \underset{f, \cn \in \mathcal{F} \times \Go}{\operatorname{arg\,min}} \cml[f, \cn]
\end{equation}
By definition, we then have
\begin{equation}
    \cml[\hat f, \hat \cn] = \underset{\cn\in\Go}{\mathrm{min}} \cml[\hat f, \cn]
    \label{eq:loss_phi_max}
\end{equation}
Using Assumption 1, we have already shown that (a) in Lemma 1 will be `=' for $\hat f$ and arbitrary $\cn$, 
the loss has its minimum possible value w.r.t.~$f$, and the bound can be reached exactly.
We use the equality to substitute $\cml$ in Eq. \ref{eq:loss_phi_max}:
\begin{equation}
    H(X|\hat \cn(Y)) = \underset{\cn\in\Go}{\mathrm{min}} H(X| \cn(Y)) 
\end{equation}
As a final step, we subtract the constant $H(X)$ to both sides.
It can be written inside the $\mathrm{min}()$ operation, 
as it does not depend on $\cn$.
Writing out the entropies and rearranging the terms directly gives
\begin{equation}
    - I(X, \hat \cn(Y)) = \underset{\cn\in\Go}{\mathrm{min}} - I(X, \cn(Y)) 
\end{equation}
\QED
\\[3mm]
\textbf{Proposition 2. }{\it
Assume $\cn$ is optimized over $\Gi$ and $\dim(C) \geq \dim(Y)$ (Assumption 3),
and $f$ is optimized over $\mathcal{F}$ (Assumption 1).
Then the following holds for $\hat f, \hat \cn \in \operatorname{arg\,min}{\cml[f, \cn]}$:
\begin{equation}
    \hat q(X | \hat \cn(Y)) = p(X|Y)
\end{equation}
}
\\[3mm]
\textbf{Proof.}
We consider the KL-divergence between the true and learned posterior,
write it out, and identify the loss and the conditional entropy:
\begin{align}
    D_\mathrm{KL}\big( p(X\mid Y) \| \hat q(X \mid \hat \cn(Y))\big) \\
    = \cml[f, \cn] - H(X\mid Y)
\end{align}
In Lemma 1, we showed that $H(X\mid Y)$ is the global minimum of the loss,
and will be reached in training under Assumptions 1, 2, and 3 ((a) and (b) both `=').
Then we can immediately see that the KL-divergence is zero, 
which is the case iff the two distributions are identical.
\QED

\section{Additional Experiments}
\subsection{Class-conditional generation for MNIST}

\noindent
To examine the behaviour of the INN without the conditioning network, we perform class-conditional generation of MNIST digits.
We construct a INN of 24 CCBs using fully connected subnetworks $s$ and $t$, 
which receive the conditioning directly as a one-hot vector.

\begin{wrapfigure}{R}{0.5\linewidth}
        \includegraphics[width=\linewidth]{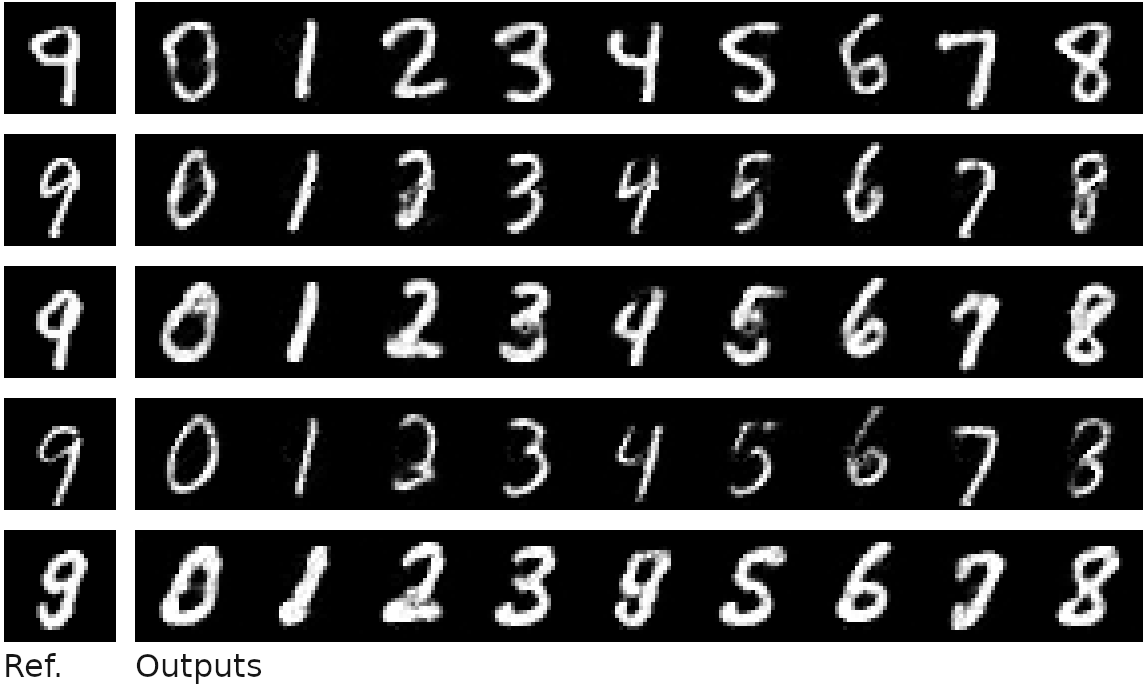}%
        \vspace{-2mm}
    	{\caption{To perform style transfer, we determine the latent code $\z = f(\x; \cond, \theta)$ of a test image \emph{(left)}, 
    	then use the inverse network $g = f^{-1}$ with different conditions ${\cond'}$ to generate the other digits in the same style, 
    	${\x'} = g(\z; {\cond'}, \theta)$.}
    	\label{fig:mnist_transfer}}
    \vspace{-3mm}
\end{wrapfigure}

Samples generated by the model are shown in \cref{fig:mnist_samples}. 
We find that the cINN learns latent representations that are shared across conditions $\cond$.
Keeping the latent vector $\z$ fixed while varying $\cond$ produces different digits in the same style.
This property, in conjunction with our network's invertibility, can directly be used for style transfer, as demonstrated in \cref{fig:mnist_transfer}.
This outcome is not obvious -- the trained cINN could also decompose into 10 essentially separate subnetworks, one for each condition.
In this case, the latent space of each class would be structured differently, and inter-class transfer of latent vectors would be meaningless.
The structure of the latent space is further illustrated in \cref{fig:mnist_attributes}, where we identify three latent axes with interpretable meanings.
Note that while the latent space is learned without supervision, we found the axes in a semi-automatic fashion:
We perform PCA on the latent vectors of the test set, without the noise augmentation, and manually identify meaningful directions in the subspace of the first four principal components.
\begin{figure}
\begin{center}
    \parbox{0.73\linewidth}{
    	{  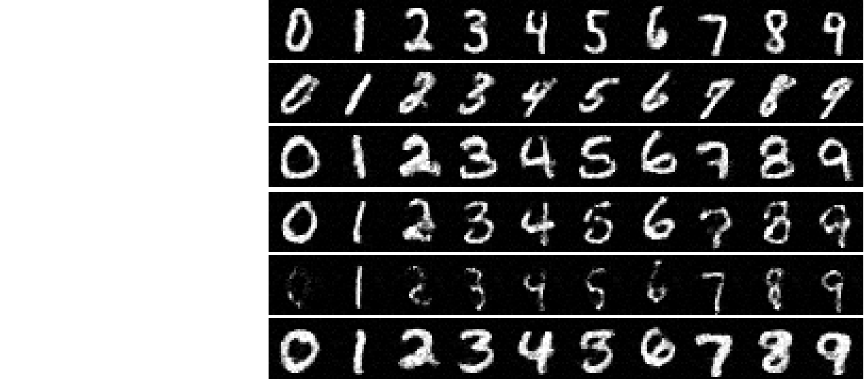 }
    	\vspace{-6mm}
    	{\caption{MNIST samples from our cINN conditioned on digit labels.
    	All ten digits within one row $(0, \dotsc, 9)$ were generated using the same latent code $\z$, but changing condition $\cond$.
    	We see that each $\z$ encodes a single style consistently across digits, while varying $\z$ between rows leads to strong differences in writing style.% \CR{line x is fat, ...}
    	} \label{fig:mnist_samples}}}
\end{center}
\end{figure}

\begin{figure}
    \centering
    \includegraphics[width=1.0\textwidth]{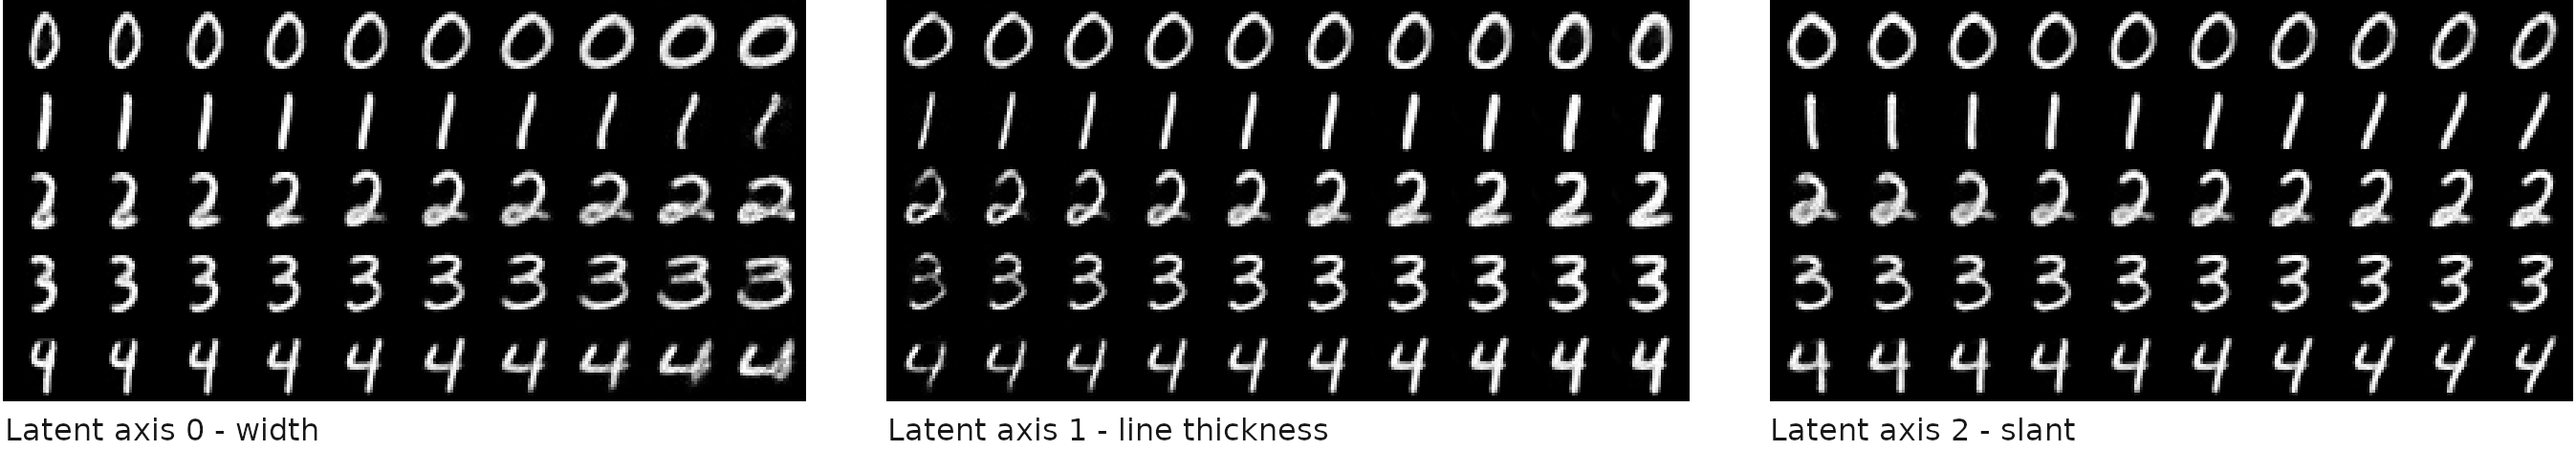}%
    \vspace{-4mm}%
	\caption{Axes in our MNIST model's latent space, which linearly encode the style attributes width, thickness and slant.}
	\vspace{-5mm}
	\label{fig:mnist_attributes}
\end{figure}

\subsection{Ablation of training improvements}
To demonstrate the improved stability and training speed through the improvements from Sec.~\ref{sec:experiments},
we perform ablations, see Fig.~\ref{fig:ablations}.
The ablations for colorization were performed for the LSUN bedrooms task, due to training speed.

We find that for stable training at Adam learning rates of $10^{-3}$, 
the tanh-clamping of $s$ and Haar wavelet downsampling are strictly necessary.
Without these, the network has to be trained with much lower learning rates and more careful and specialized initialization, 
as used e.g. in \cite{kingma2018glow}.
Beyond this, the noise augmentation and permutations lead to the largest improvement in final result.
The effect of the noise is more pronounced for MNIST, possibly becuase large parts of the image are completely black otherwise,
additionally leading to a problem with sparse gradients.
%For natural images, dequantization of the data is likely to be the main advantage of the added noise.
Note however, that the training curves of the models with and without noise augmentation is not directly comparable,
as the loss differs an additional summand $\approx \log(\sigma_\mathrm{aug.})$. 
The effect on the training speed and stability is clearly visible regardless.
The initialization only improves the final result by a small margin, but also converges noticeably faster.

\begin{figure}[h]
    \centering
    \includegraphics[width=0.49\linewidth]{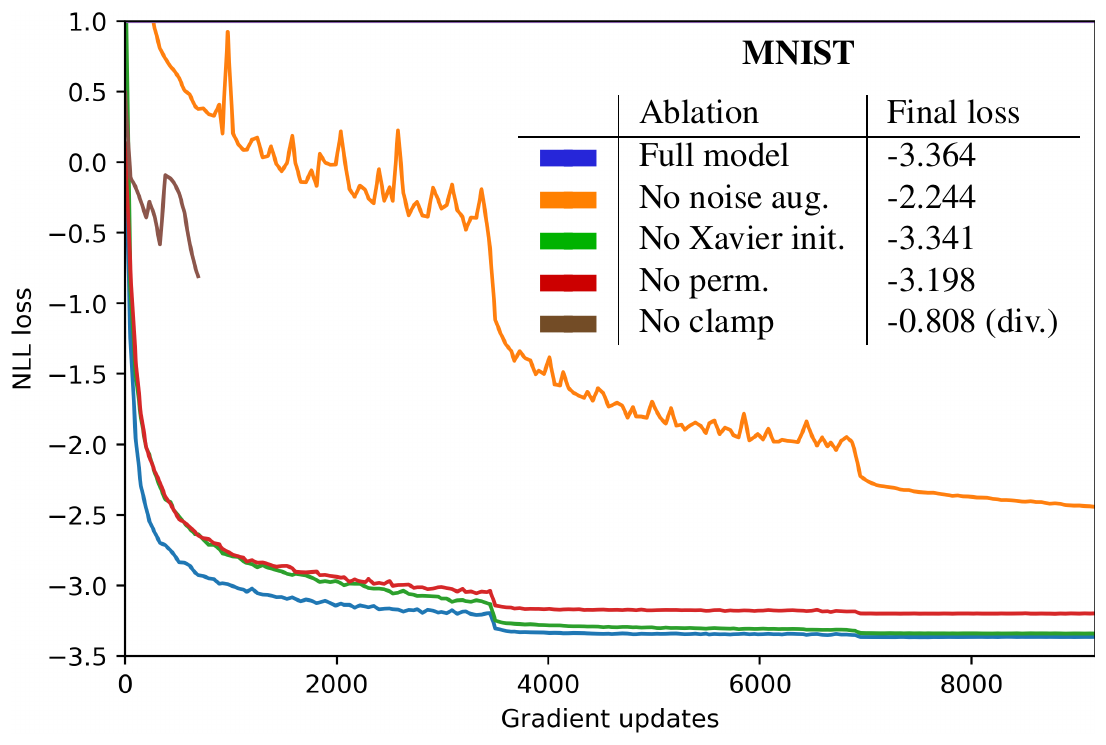}%
    \includegraphics[width=0.49\linewidth]{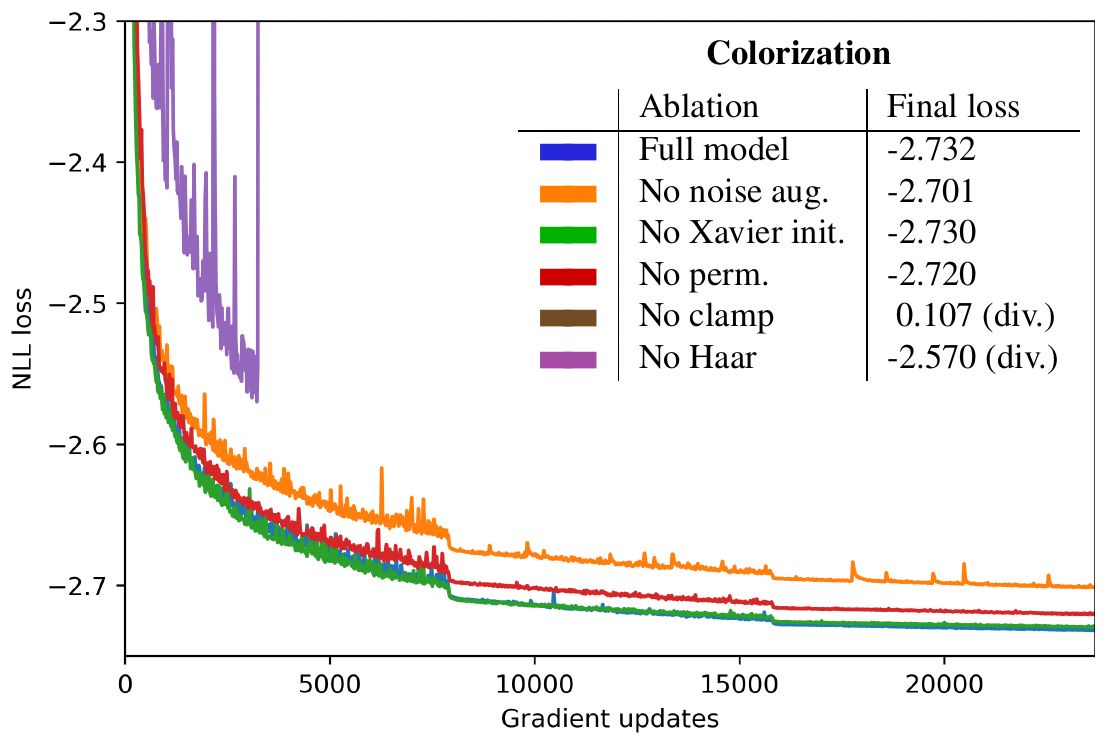}
    \caption{Training curves for each task, ablating the different improvements. "div." denotes that the training diverges, and the lowest loss so far is given.}
        \label{fig:ablations}
\end{figure}

\subsection{LSUN Bedrooms}
To provide a simpler model for more in-depth experiments and ablations,
we additionally train a cINN for colorization on the LSUN bedrooms dataset \cite{yu2015lsun}.
We use a smaller model than for ImageNet, and train the conditioning network
jointly from scratch, without pretraining. 
Both the conditioning input, as well as the generated color channels have a resolution of $64\times 64$ pixels.
The entire model trains in under 4 hours on a single GTX 1080Ti GPU.

To our knowledge, the only diversity-enforcing cGAN architecture previously used 
for colorization is the colorGAN \cite{cao2017unsupervised}, 
which is also trained exclusively on the bedrooms dataset.
Training the colorGAN for comparison, we find 
it requires over 24 hours to converge stably, after multiple restarts.
The results are generally worse than those of the cINN,
as shown in Fig.~\ref{fig:colorgan}.
While the resulting pixel-wise color variance is slightly higher for the colorGAN, 
it is not clear whether this captures the true variance, 
or whether it is due to unrealistically colorful outputs, such as in the second row in Fig.~\ref{fig:colorgan}.

\begin{table}[h]
    \centering
    \begin{tabular}{l | r | r}
        Metric & cINN & colorGAN \\
        \hline
        MSE best-of-8 &  \bftab 6.14  & 6.43  \\
        Variance      &  33.69 & \bftab 39.46 \\
        FID           & \bftab 26.48 & 28.31\\
    \end{tabular}

    \caption{Quantitative comparison between smaller cINN and colorGAN on LSUN bedrooms.
    The metrics used are explained in Table \ref{tab:results}.}
\end{table}

\begin{figure}
    \begin{center}
    \begin{tabular}{p{0.49\linewidth} p{0.49\linewidth}}
        cINN & COLORGAN
    \end{tabular}
    
    \includegraphics[width=\linewidth]{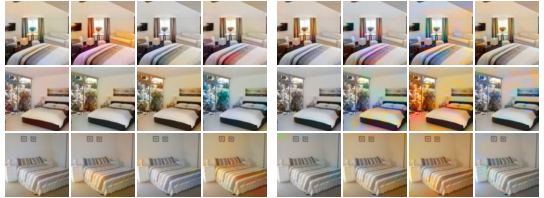}
    \end{center}
    \caption{Qualitative comparison between smaller cINN and colorGAN on LSUN bedrooms.}
    \label{fig:colorgan}
\end{figure}

%\bibliographystyle{splncs03}
%\bibliography{bibliography}

\section{Additional Figures}

% \begin{figure}[h]
%     \vspace{-3mm}
%     \centering
%     %\includegraphics[width=\textwidth]{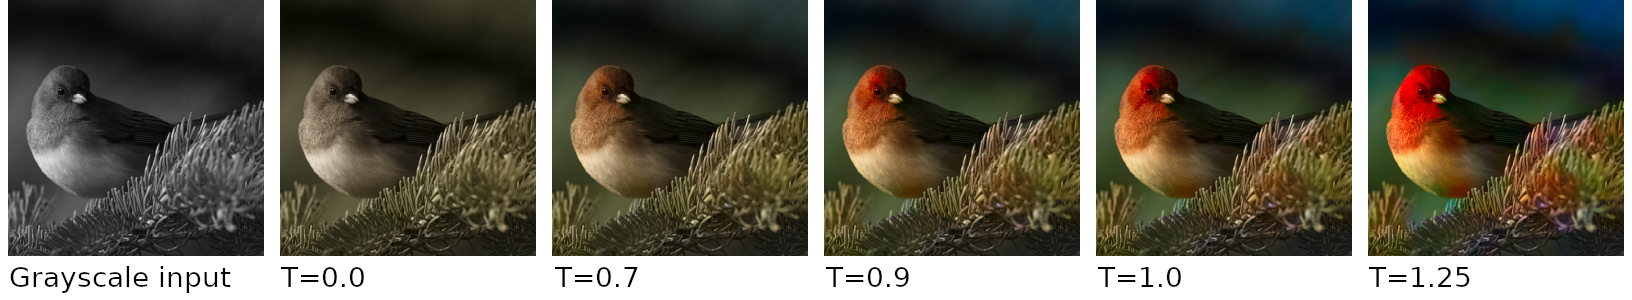}
% 	{ \def\svgwidth{\textwidth} \input{figures/temperatures.tex} }
%     \includegraphics[width=\textwidth]{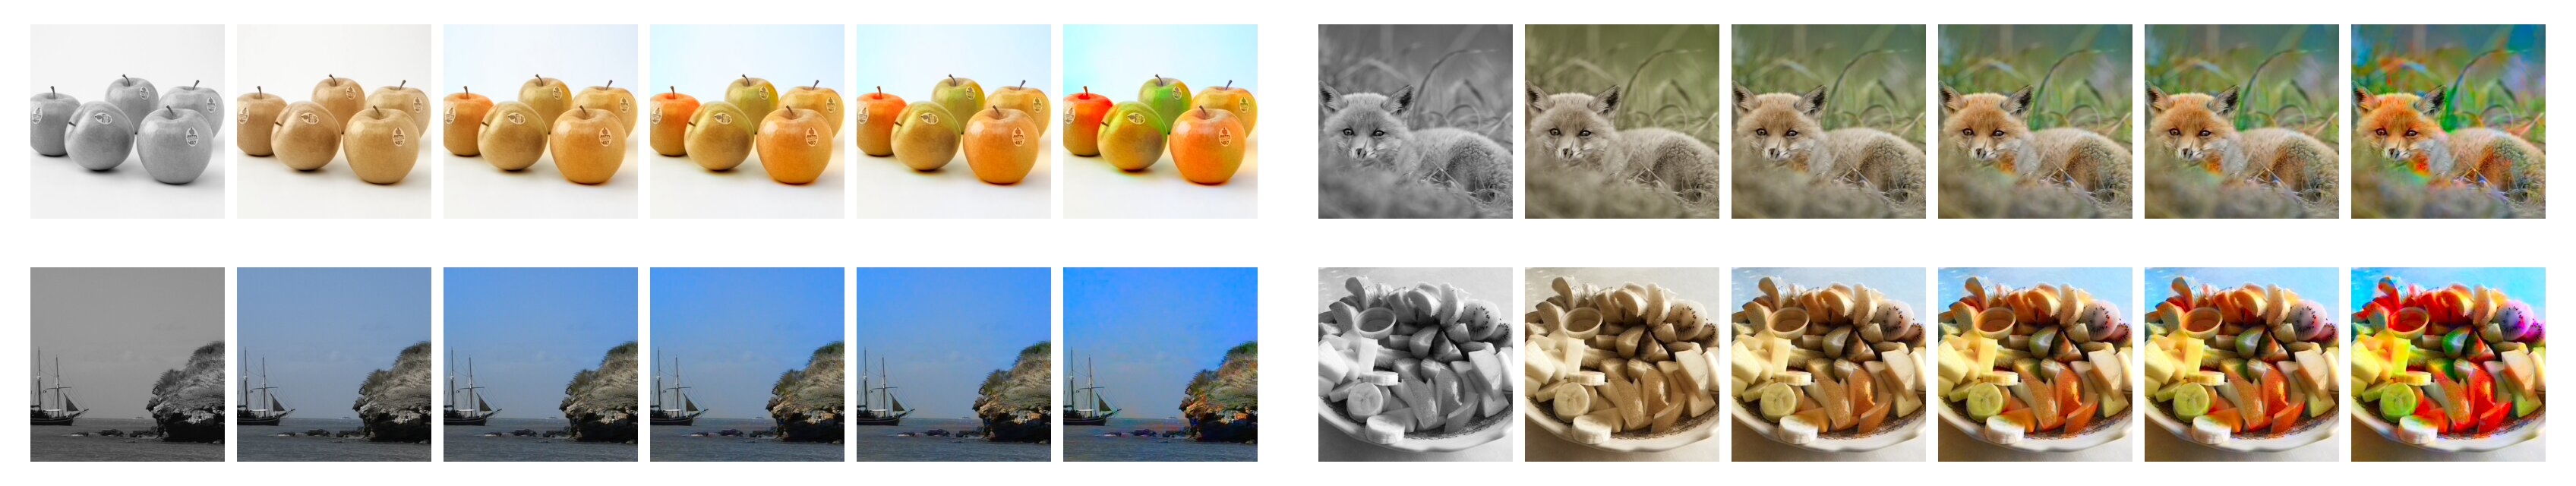}
% 	\caption{Effects of linearly scaling the latent code $\z$ while keeping the condition fixed.
% 	Vector $\z^*$ is ``typical'' in the sense that $\|\z^*\|^2=\mathbb{E}\big[\|\z\|^2\big]$, and results in natural colors.
% 	As we move closer to the center of the latent space ($\|\z\| < \|\z^*\|$), regions with ambiguous colors become desaturated, while less ambiguous regions (e.g.~sky, vegetation) revert to their prototypical colors.
% 	In the opposite direction ($\|\z\| > \|\z^*\|$), colors are enhanced to the point of oversaturation.
% 	\vspace{-4mm}
% 	}
% 	\label{fig:latent_temperature}
% \end{figure}

\subsection{Colorization -- Interpolations}
In the following, we show 2-dimensional interpolations in latent space.
Two random latent vectors $\z^{(1)}$, $\z^{(2)}$ are linearly combined:
$$    \z^* = a_1 \z^{(1)} + a_2 \z^{(2)} $$
with varying $a_1$, $a_2 \in [-0.9 \dots 0.9]$ across each axis of a grid.
The center image has $\z^*=0$.
Note that the images in the corners have a larger magnitude 
than trained for, $\|z^*\|_2 \approx 1.3 \, \mathbb{E}\big[\|\z\|_2\big]$, 
leading to some oversaturation artifacts, as in Fig.~12 of the main paper.

\begin{figure*}
\centering
\includegraphics[width=1.0\textwidth]{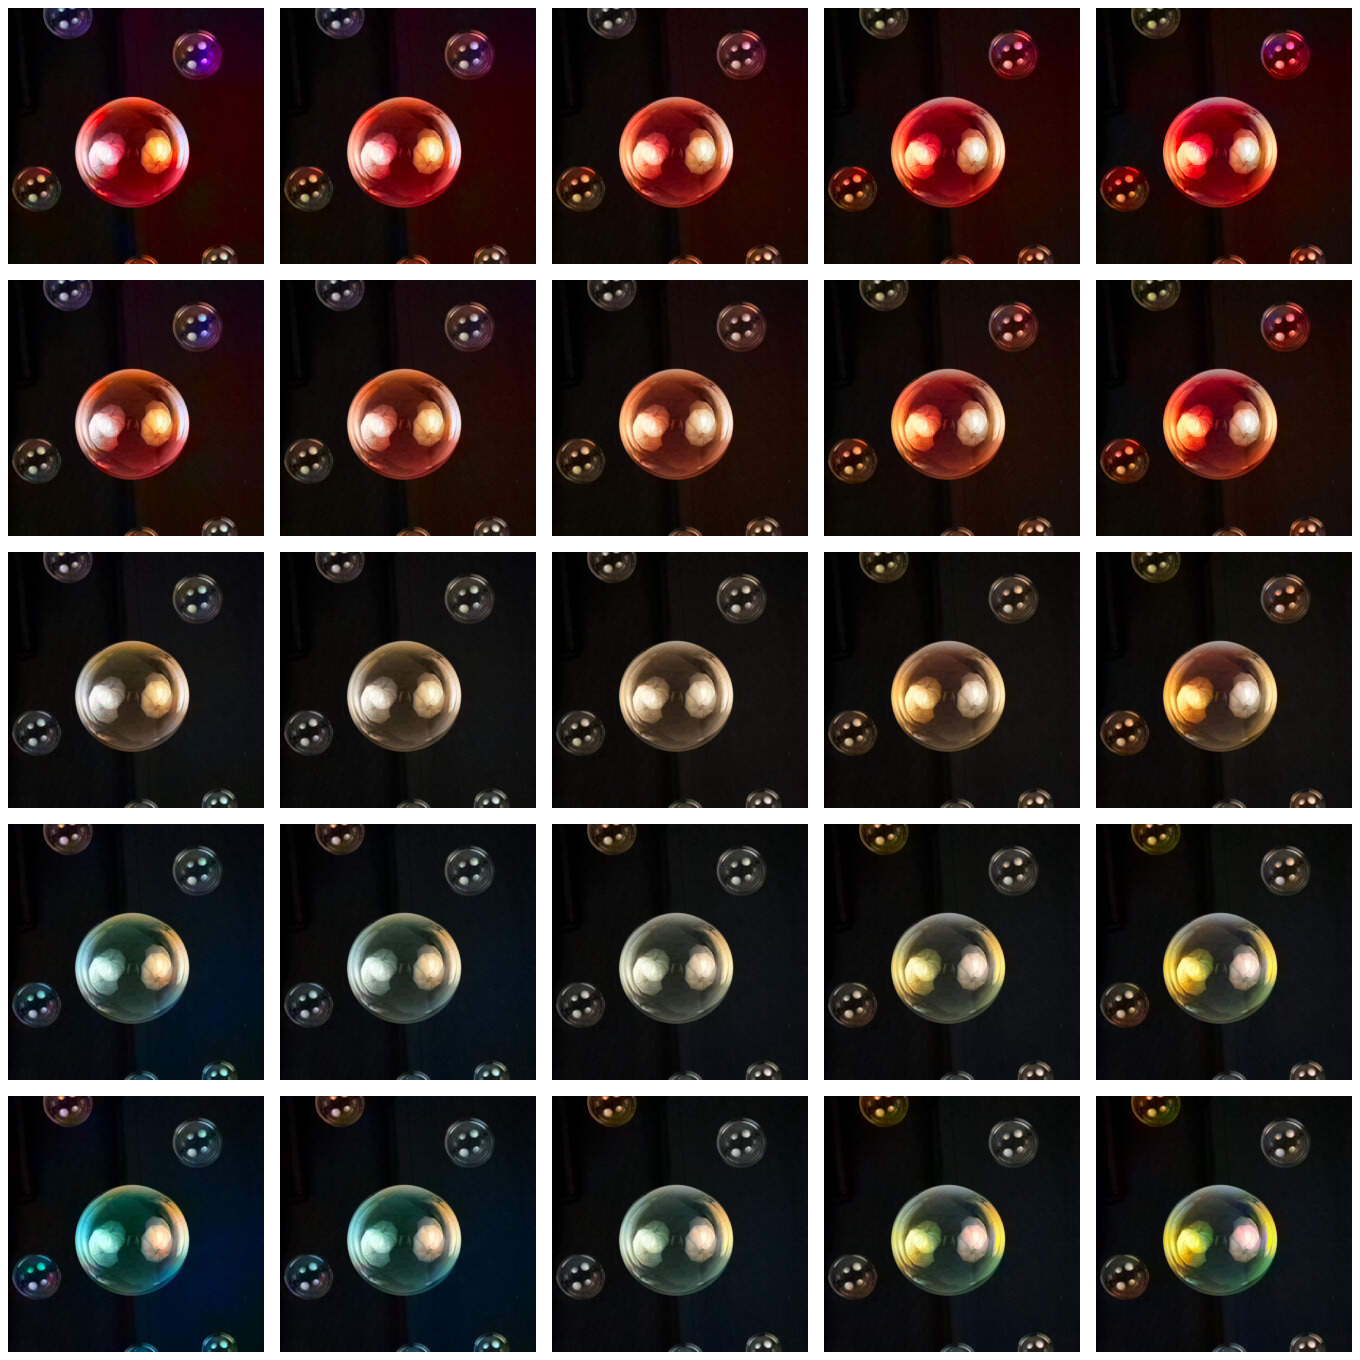} 
\end{figure*}

\begin{figure*}
\centering
\includegraphics[width=1.0\textwidth]{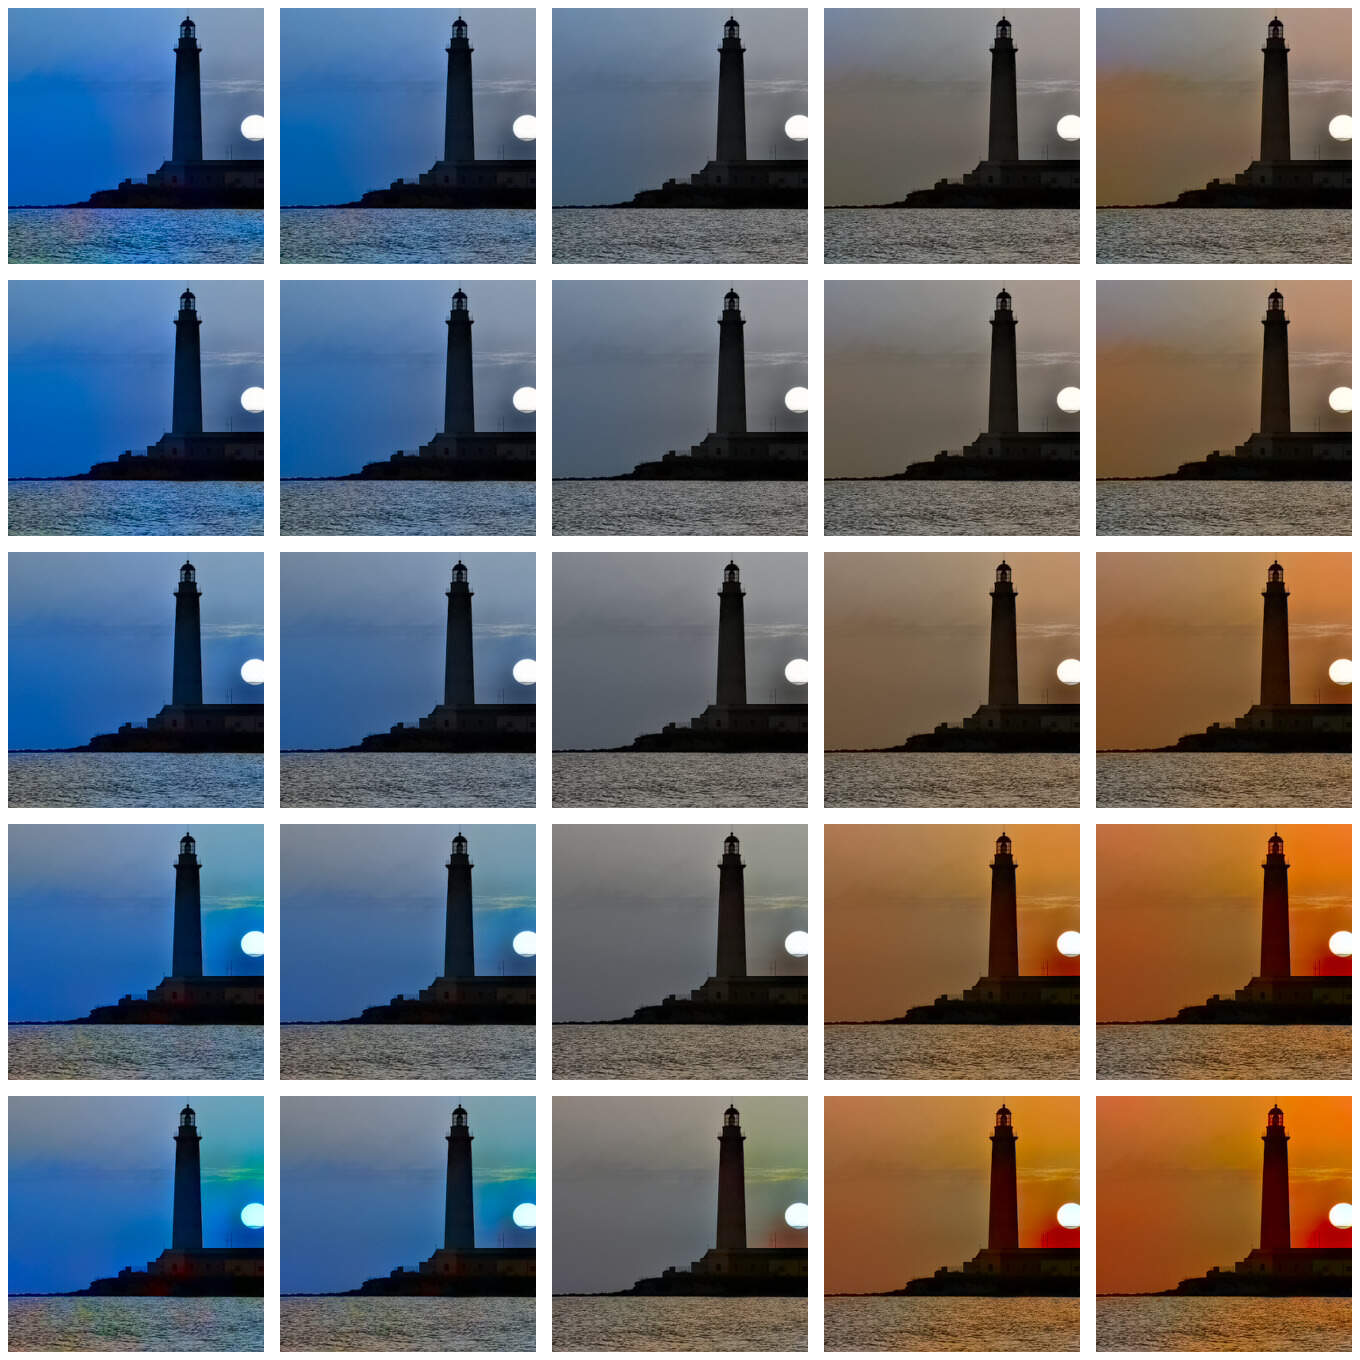} 
\end{figure*}

\begin{figure*}
\centering
\includegraphics[width=1.0\textwidth]{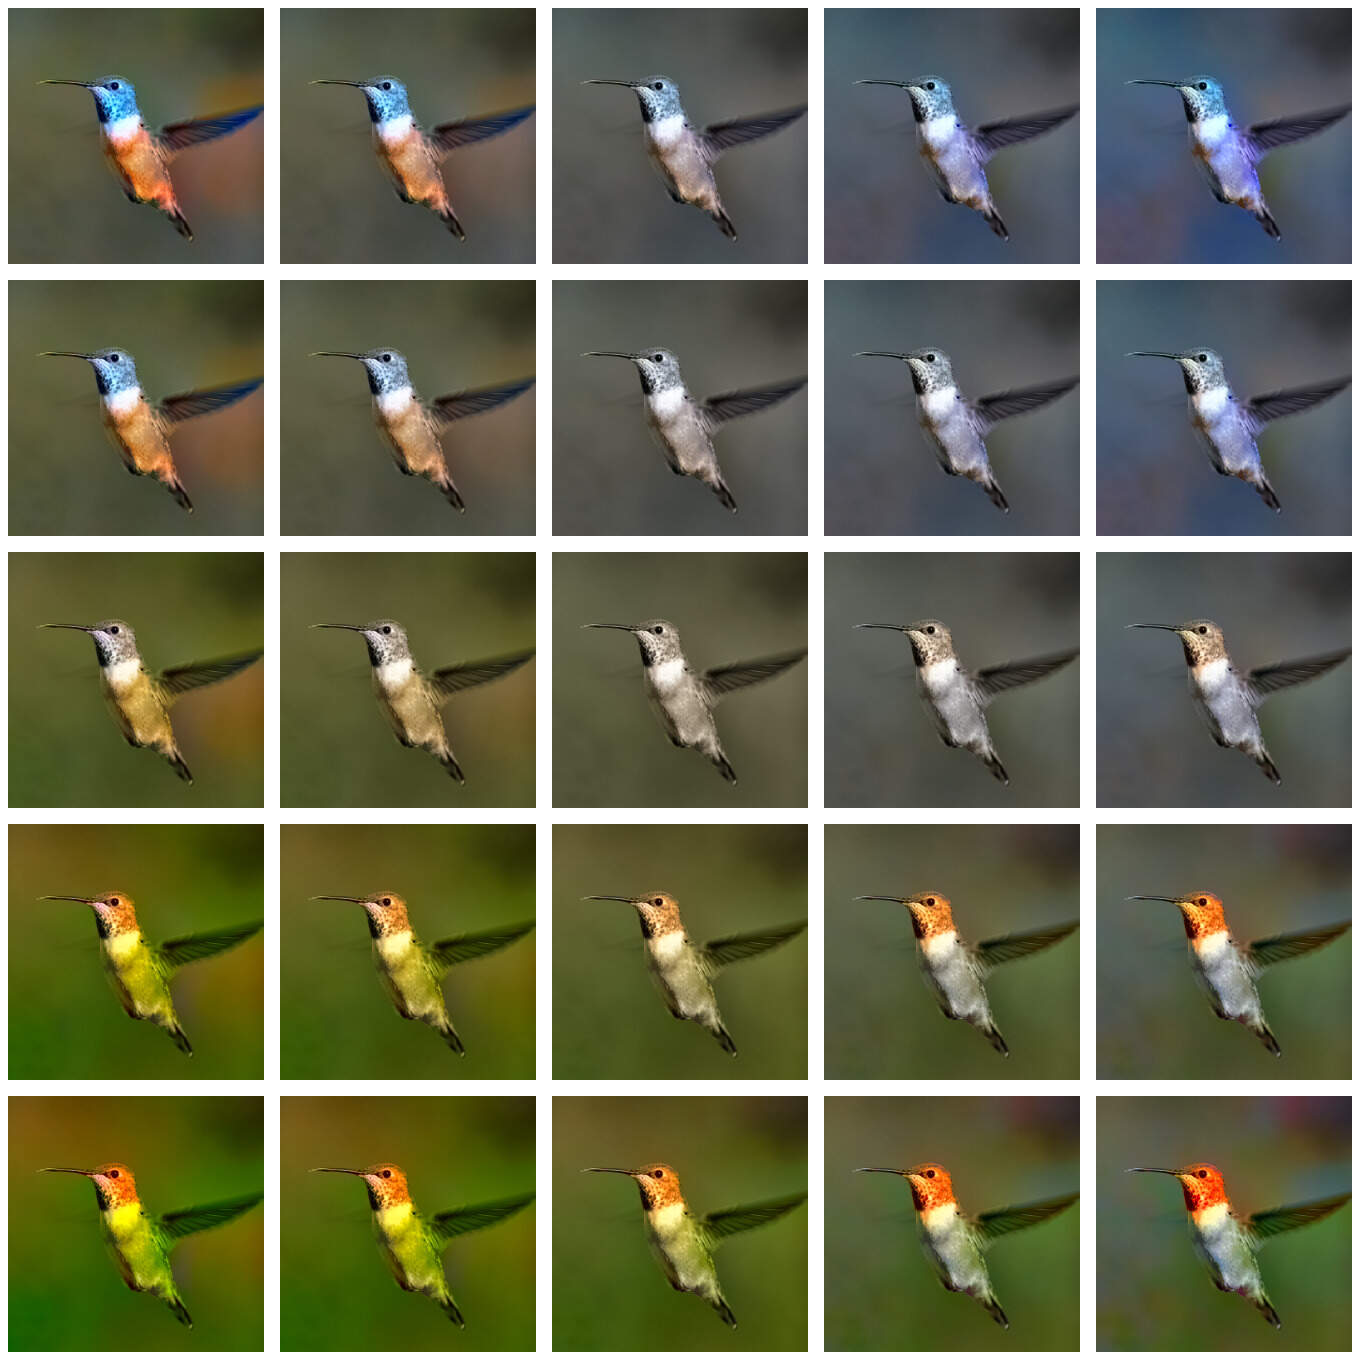} 
\end{figure*}

\begin{figure}
\centering
\includegraphics[width=1.0\textwidth]{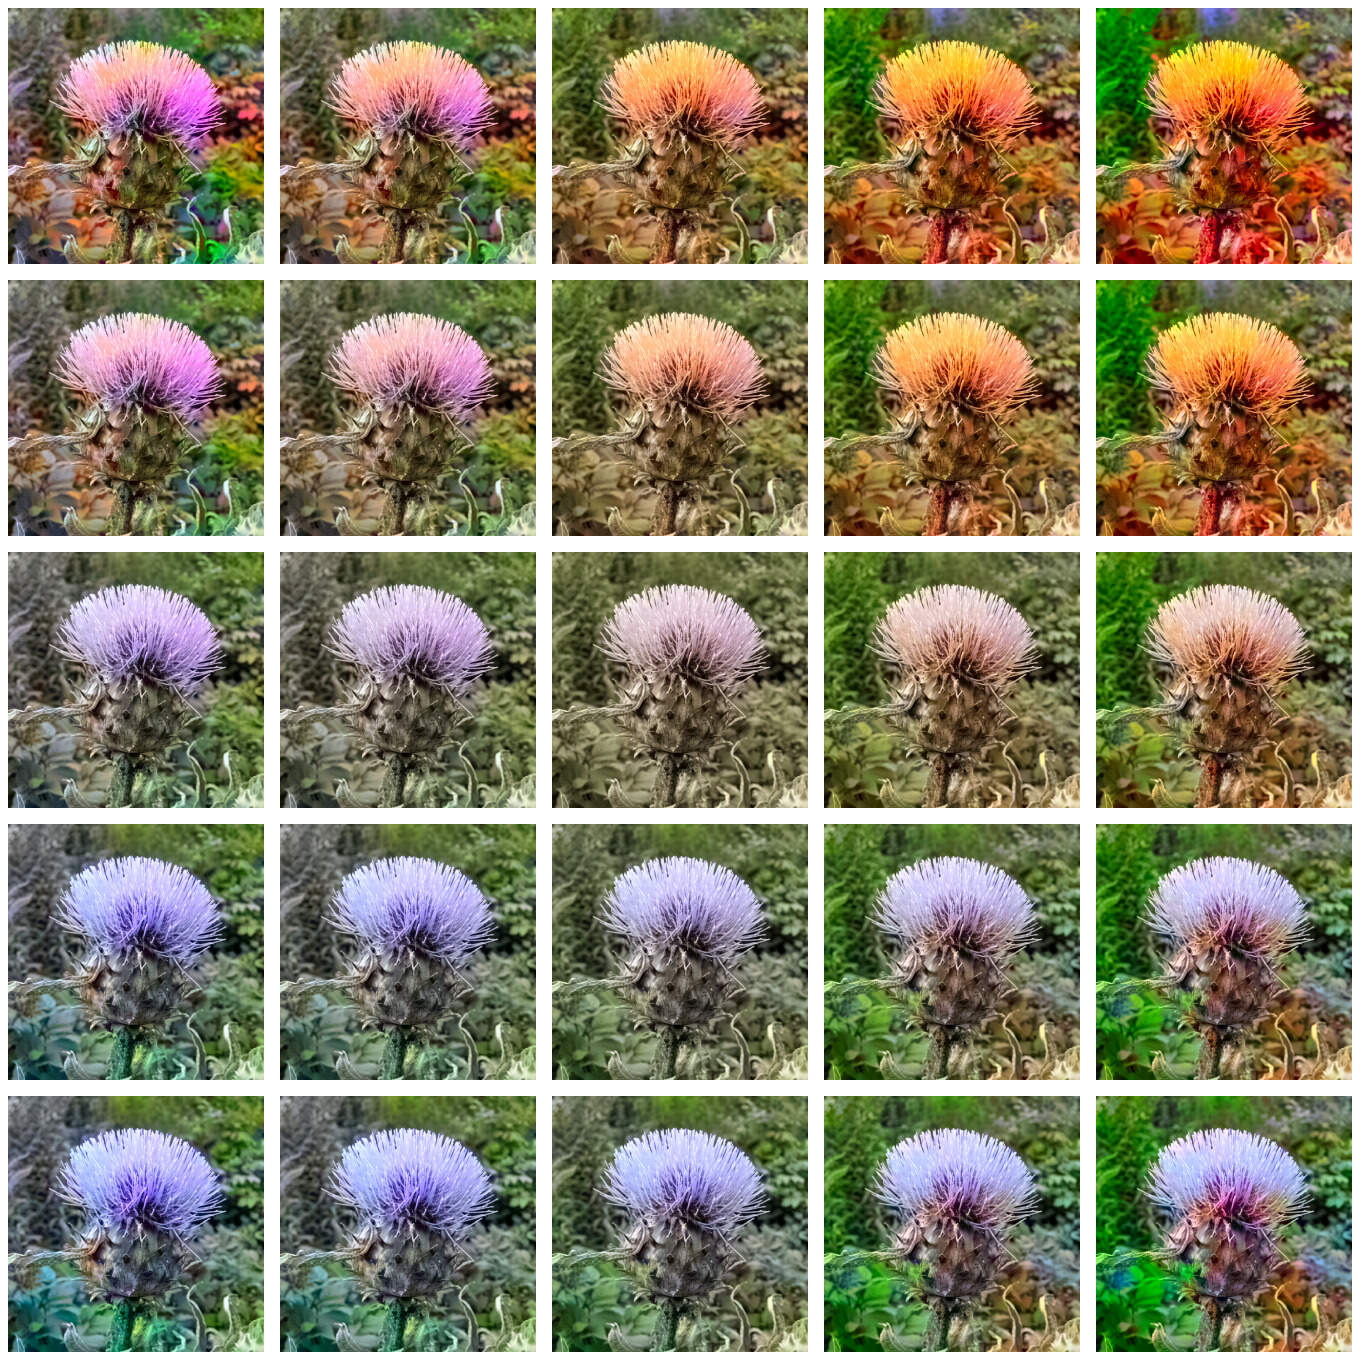} 
\end{figure}

\begin{figure*}
\centering
\includegraphics[width=1.0\textwidth]{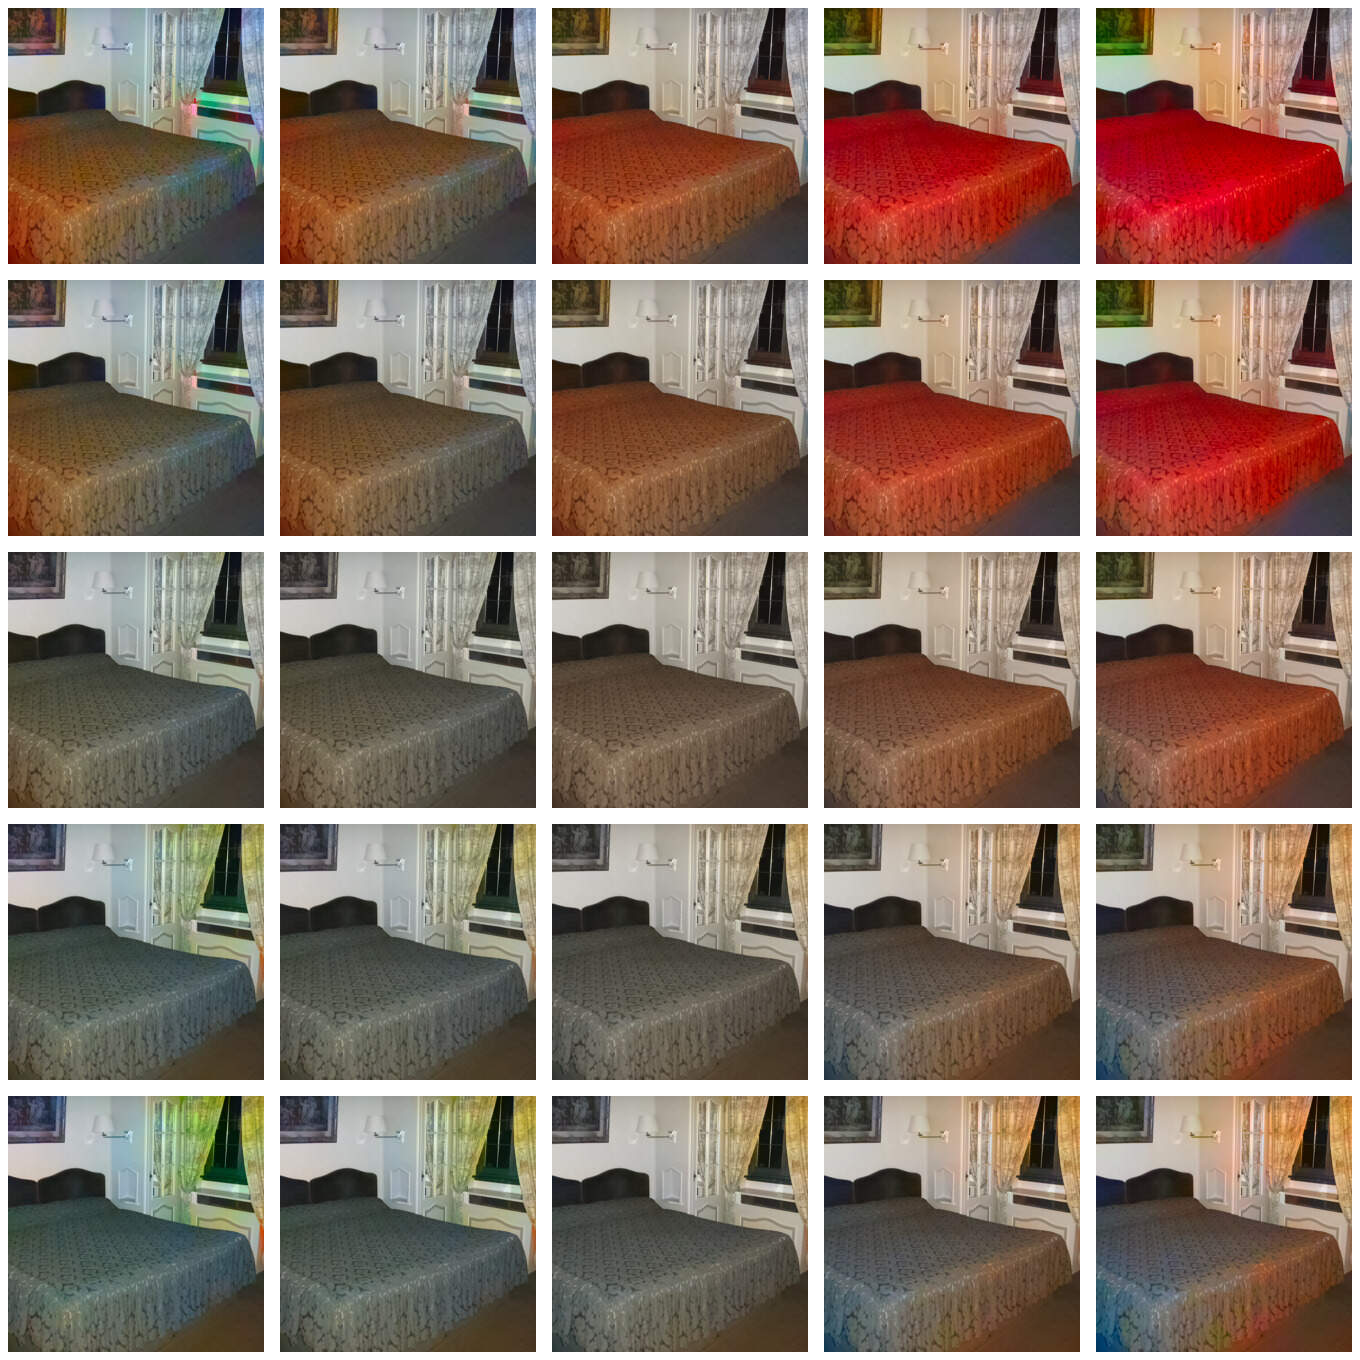} 
\end{figure*}

\FloatBarrier
%   
%   % TODO not in overleaf, because too big
%   \subsection{Colorization -- Additional examples}
%   \noindent
%   On the following pages, we provide some additional colorized images, as well as comparisons to alternative methods.
%   All images are taken from the ImageNet 2012 validation set, and all methods were trained on ImageNet 2012.
%   As we do not observe any significant diversity for the cGAN, we only provide a single sample.
%   
%   \subsubsection{General examples}
%   
%   \subsubsection{Humans}
%   \noindent
%   We find that the cINN often has difficulties generating convincing skin colors, as shown below.
%   Clothing is colored in diverse ways, but not always with the correct connectivity and consistency.
%   
%   \subsubsection{Lacking consistency}
%   \noindent
%   The following failure cases exhibit a lack in consistency, in occluded objects, multi-part objects, or reflections.
%   
%   \subsubsection{Color ignores semantic content}
%   \noindent
%   In the following examples, the semantic content of the image was not recognized, and the generated colors are clearly incorrect.
%   
%   \subsubsection{Outright failures}
%   \noindent
%   For the following images, the cINN fails completely, and generates colors with seemingly little or no connection to the grayscale image.
