# Supplementary material for: Conditional Invertible Neural Networks for Diverse Image-to-Image Translation
Source: arXiv:2105.02104 source file (2021-05-05)
Supplement: Supplementary file 2 [file 05_appendix.tex]

\subsection{Ablation of training improvements}
To demonstrate the improved stability and training speed through the improvements from Sec.~\ref{sec:experiments},
we perform ablations, see Fig.~\ref{fig:ablations}.
The ablations for colorization were performed for the LSUN bedrooms task, due to training speed.

We find that for stable training at Adam learning rates of $10^{-3}$, 
the tanh-clamping of $s$ and Haar wavelet downsampling are strictly necessary.
Without these, the network has to be trained with much lower learning rates and more careful and specialized initialization, 
as used e.g. in \cite{kingma2018glow}.
Beyond this, the noise augmentation and permutations lead to the largest improvement in final result.
The effect of the noise is more pronounced for MNIST, possibly becuase large parts of the image are completely black otherwise,
additionally leading to a problem with sparse gradients.
%For natural images, dequantization of the data is likely to be the main advantage of the added noise.
Note however, that the training curves of the models with and without noise augmentation is not directly comparable,
as the loss differs an additional summand $\approx \log(\sigma_\mathrm{aug.})$. 
The effect on the training speed and stability is clearly visible regardless.
The initialization only improves the final result by a small margin, but also converges noticeably faster.

\begin{figure}[h]
    \centering
    \includegraphics[width=0.49\linewidth]{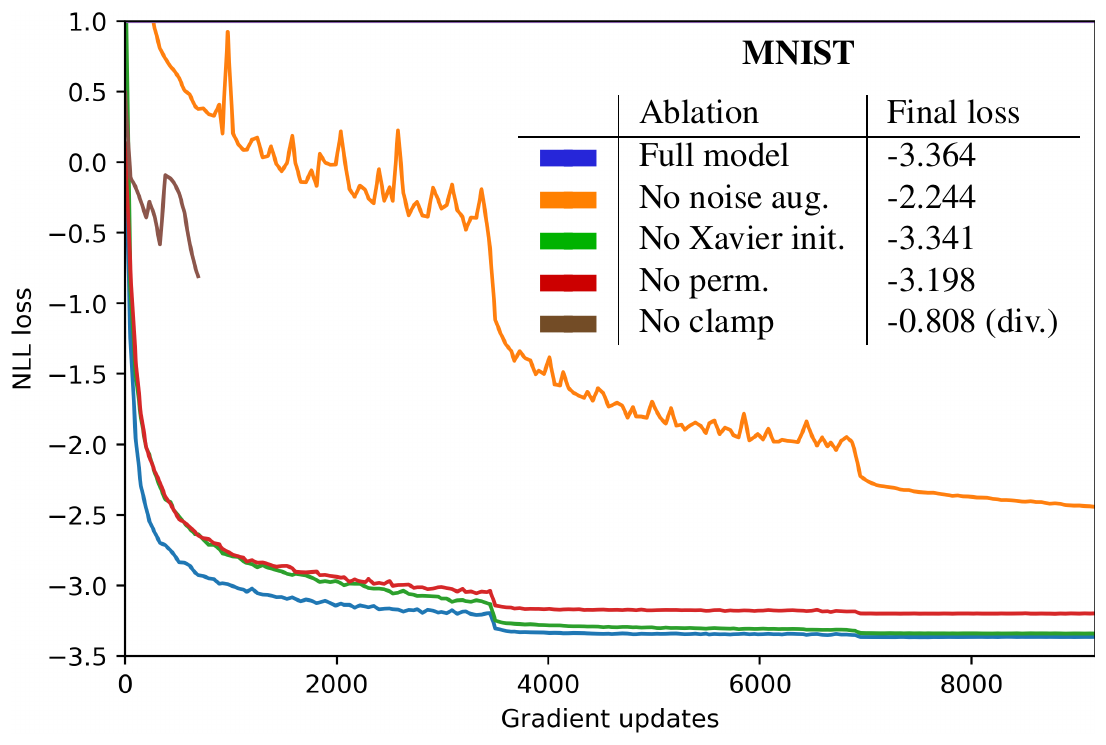}%
    \includegraphics[width=0.49\linewidth]{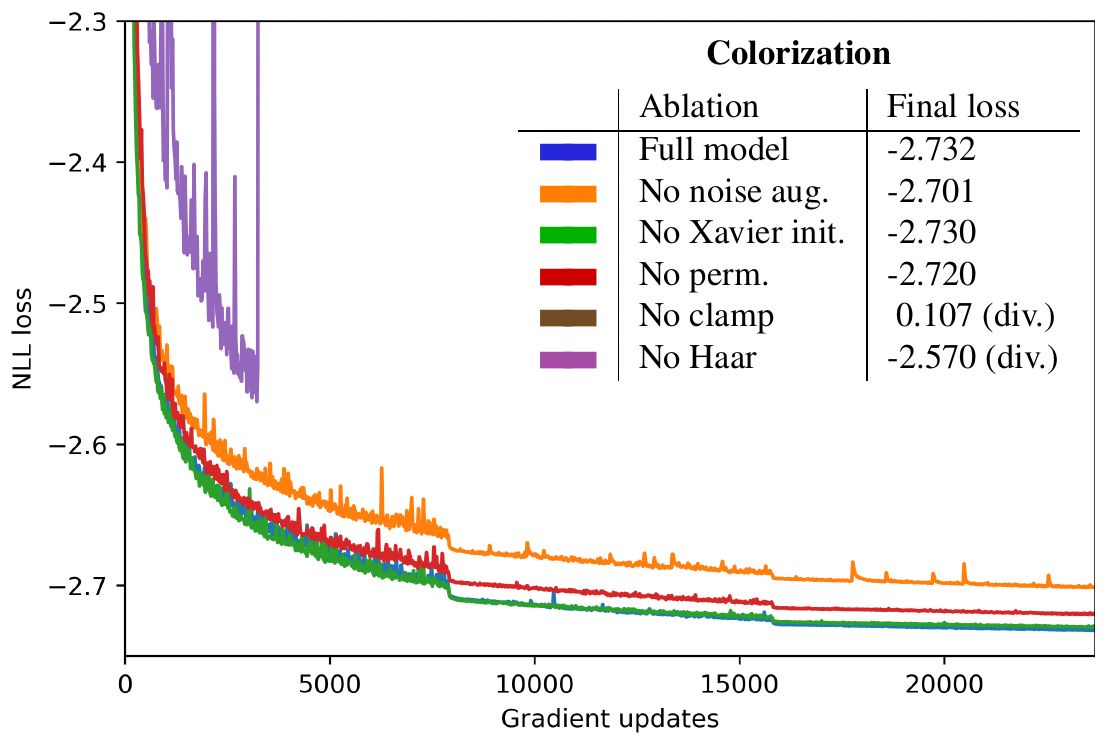}
    \caption{Training curves for each task, ablating the different improvements. "div." denotes that the training diverges, and the lowest loss so far is given.}
        \label{fig:ablations}
\end{figure}

\subsection{LSUN Bedrooms}
To provide a simpler model for more in-depth experiments and ablations,
we additionally train a cINN for colorization on the LSUN bedrooms dataset \cite{yu2015lsun}.
We use a smaller model than for ImageNet, and train the conditioning network
jointly from scratch, without pretraining. 
Both the conditioning input, as well as the generated color channels have a resolution of $64\times 64$ pixels.
The entire model trains in under 4 hours on a single GTX 1080Ti GPU.

To our knowledge, the only diversity-enforcing cGAN architecture previously used 
for colorization is the colorGAN \cite{cao2017unsupervised}, 
which is also trained exclusively on the bedrooms dataset.
Training the colorGAN for comparison, we find 
it requires over 24 hours to converge stably, after multiple restarts.
The results are generally worse than those of the cINN,
as shown in Fig.~\ref{fig:colorgan}.
While the resulting pixel-wise color variance is slightly higher for the colorGAN, 
it is not clear whether this captures the true variance, 
or whether it is due to unrealistically colorful outputs, such as in the second row in Fig.~\ref{fig:colorgan}.

\begin{table}[h]
    \centering
    \begin{tabular}{l | r | r}
        Metric & cINN & colorGAN \\
        \hline
        MSE best-of-8 &  \bftab 6.14  & 6.43  \\
        Variance      &  33.69 & \bftab 39.46 \\
        FID           & \bftab 26.48 & 28.31\\
    \end{tabular}

    \caption{Quantitative comparison between smaller cINN and colorGAN on LSUN bedrooms.
    The metrics used are explained in Table \ref{tab:results}.}
\end{table}

\begin{figure}
    \begin{center}
    \begin{tabular}{p{0.49\linewidth} p{0.49\linewidth}}
        cINN & COLORGAN
    \end{tabular}
    
    \includegraphics[width=\linewidth]{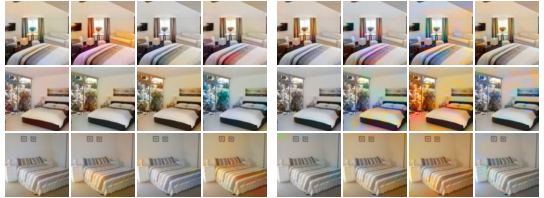}
    \end{center}
    \caption{Qualitative comparison between smaller cINN and colorGAN on LSUN bedrooms.}
    \label{fig:colorgan}
\end{figure}
