# Supplementary material for: Conditional Invertible Neural Networks for Diverse Image-to-Image Translation
Source: arXiv:2105.02104 source file (2021-05-05)
Supplement: Supplementary file 3 [file 05_appendix_images.tex]

\section{Additional Figures}

% \begin{figure}[h]
%     \vspace{-3mm}
%     \centering
%     %\includegraphics[width=\textwidth]{figures/temperatures.jpg}
% 	{ \def\svgwidth{\textwidth} \input{figures/temperatures.tex} }
%     \includegraphics[width=\textwidth]{figures/temperature_additional.jpg}
% 	\caption{Effects of linearly scaling the latent code $\z$ while keeping the condition fixed.
% 	Vector $\z^*$ is ``typical'' in the sense that $\|\z^*\|^2=\mathbb{E}\big[\|\z\|^2\big]$, and results in natural colors.
% 	As we move closer to the center of the latent space ($\|\z\| < \|\z^*\|$), regions with ambiguous colors become desaturated, while less ambiguous regions (e.g.~sky, vegetation) revert to their prototypical colors.
% 	In the opposite direction ($\|\z\| > \|\z^*\|$), colors are enhanced to the point of oversaturation.
% 	\vspace{-4mm}
% 	}
% 	\label{fig:latent_temperature}
% \end{figure}

\subsection{Colorization -- Interpolations}
In the following, we show 2-dimensional interpolations in latent space.
Two random latent vectors $\z^{(1)}$, $\z^{(2)}$ are linearly combined:
$$    \z^* = a_1 \z^{(1)} + a_2 \z^{(2)} $$
with varying $a_1$, $a_2 \in [-0.9 \dots 0.9]$ across each axis of a grid.
The center image has $\z^*=0$.
Note that the images in the corners have a larger magnitude 
than trained for, $\|z^*\|_2 \approx 1.3 \, \mathbb{E}\big[\|\z\|_2\big]$, 
leading to some oversaturation artifacts, as in Fig.~12 of the main paper.

\begin{figure*}
\centering
\includegraphics[width=1.0\textwidth]{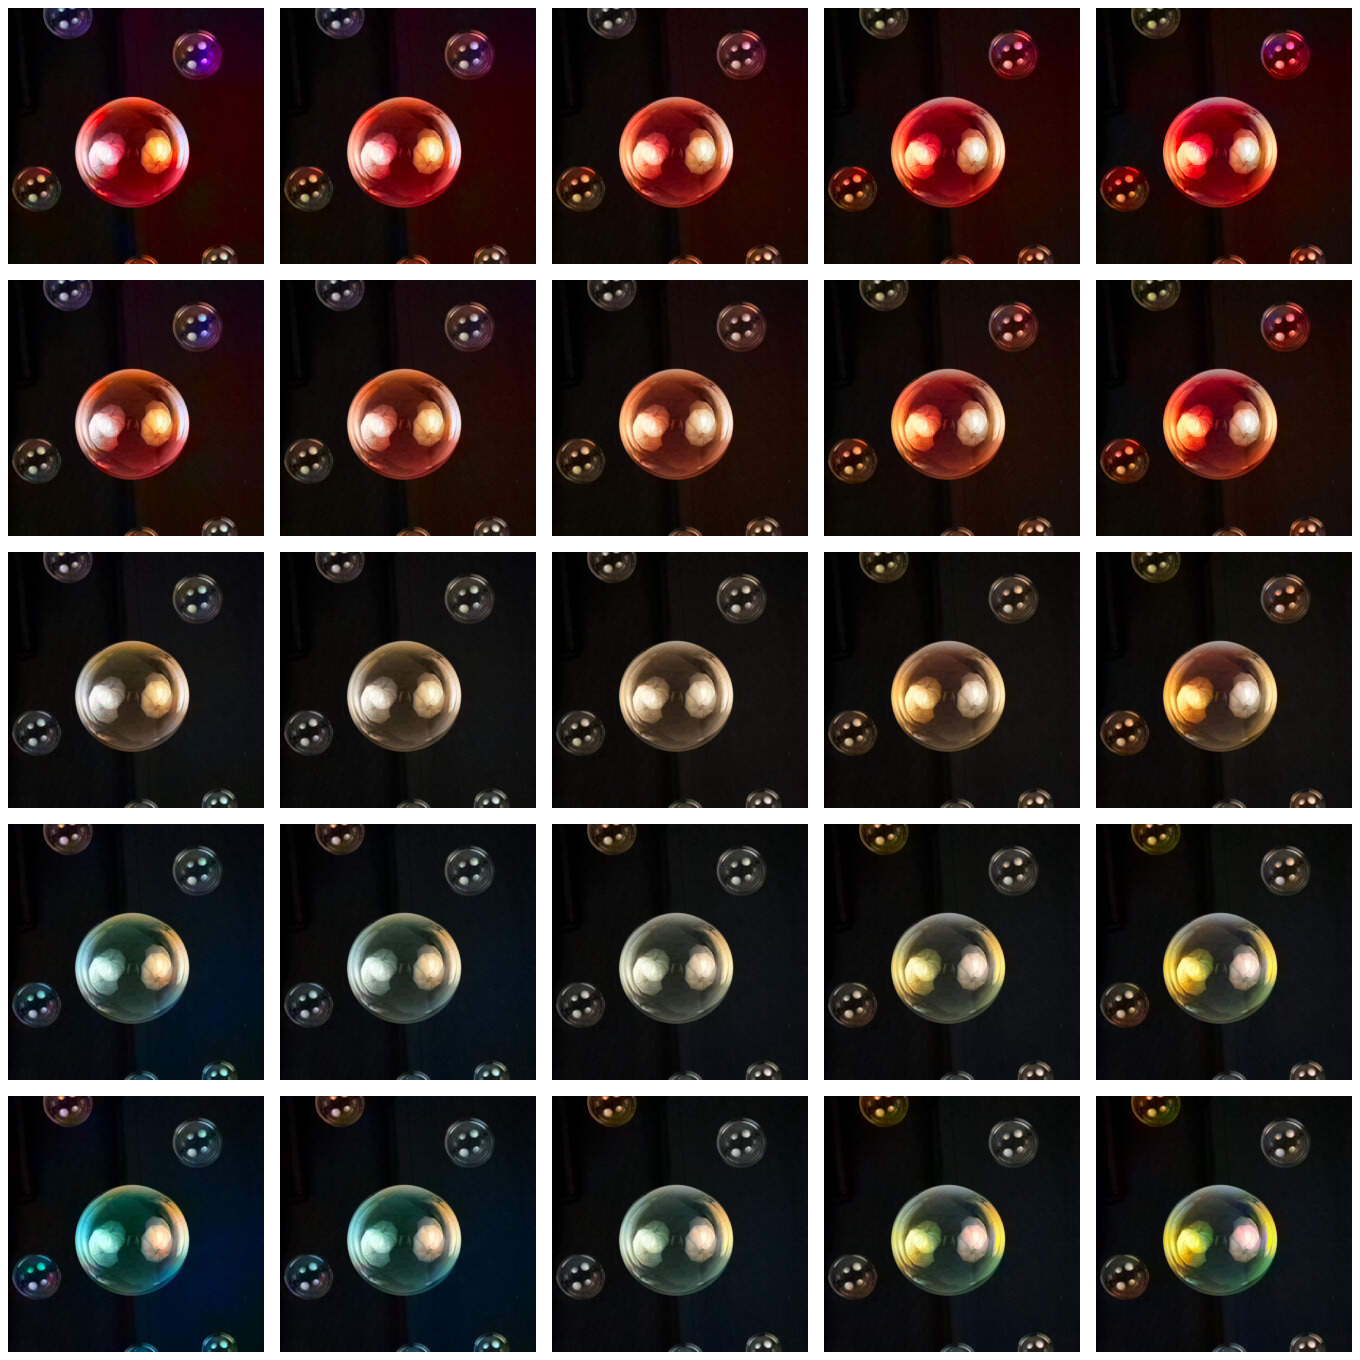} 
\end{figure*}

\begin{figure*}
\centering
\includegraphics[width=1.0\textwidth]{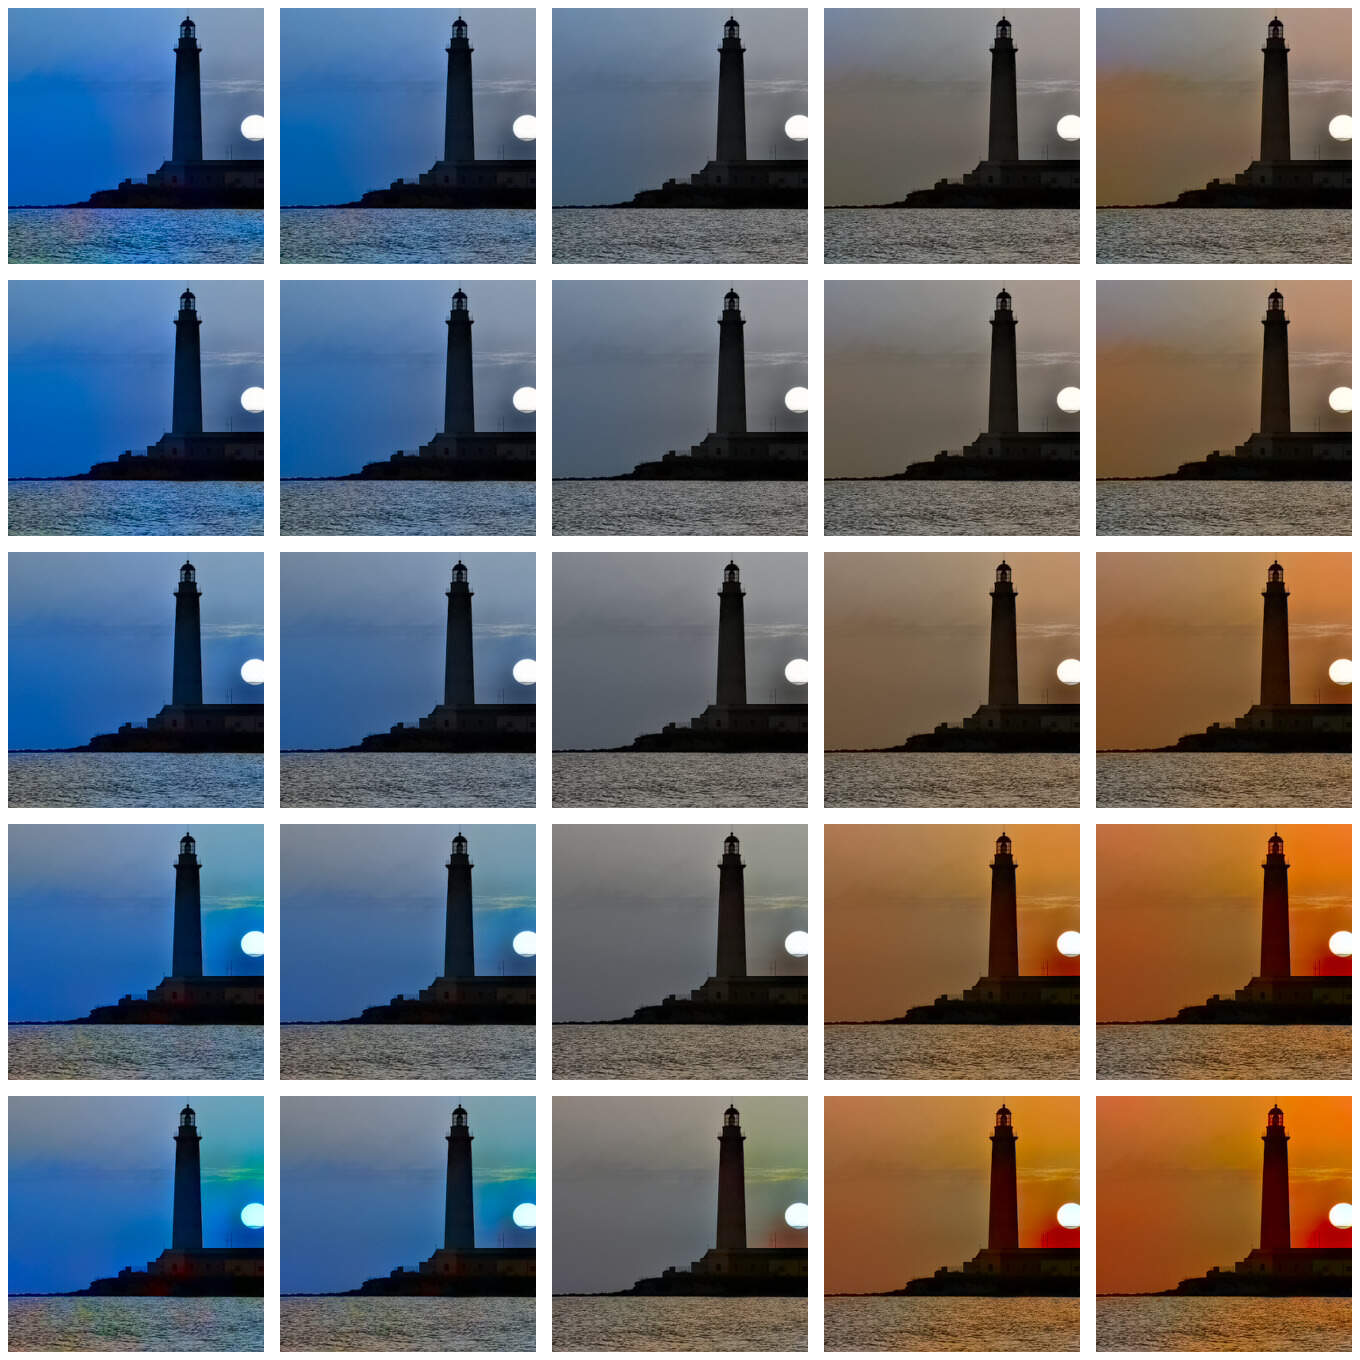} 
\end{figure*}

\begin{figure*}
\centering
\includegraphics[width=1.0\textwidth]{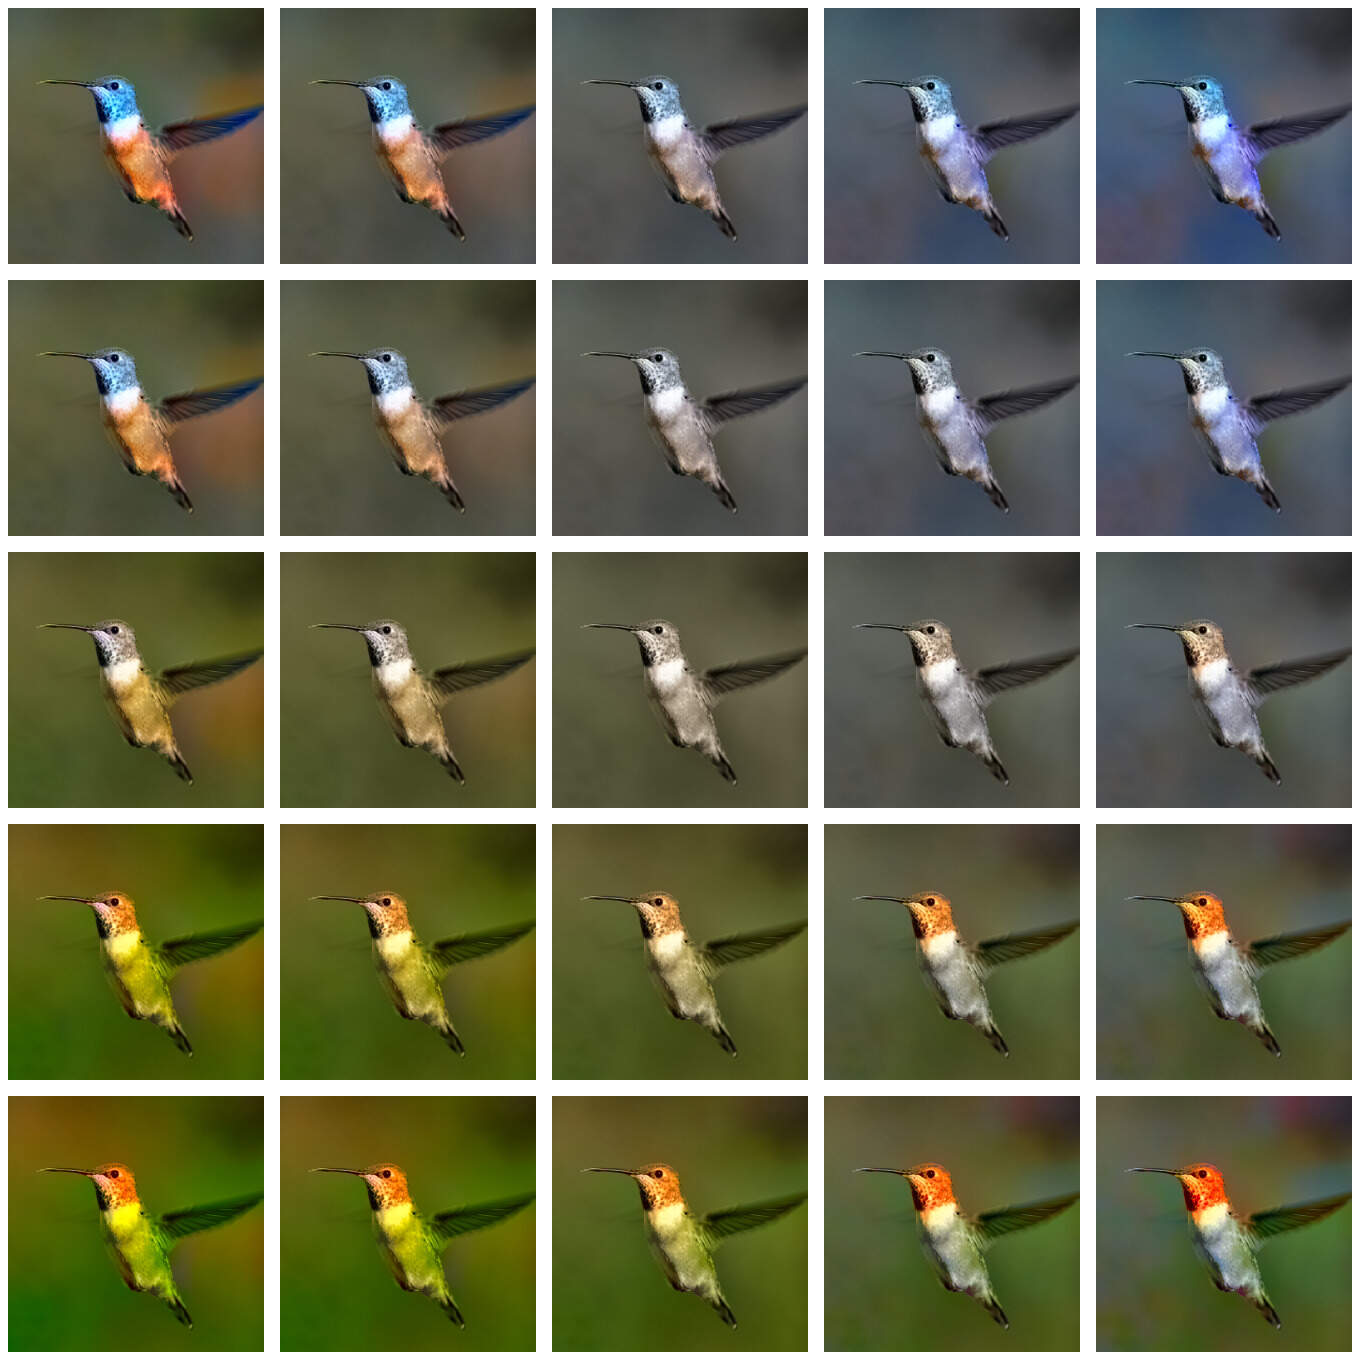} 
\end{figure*}

\begin{figure}
\centering
\includegraphics[width=1.0\textwidth]{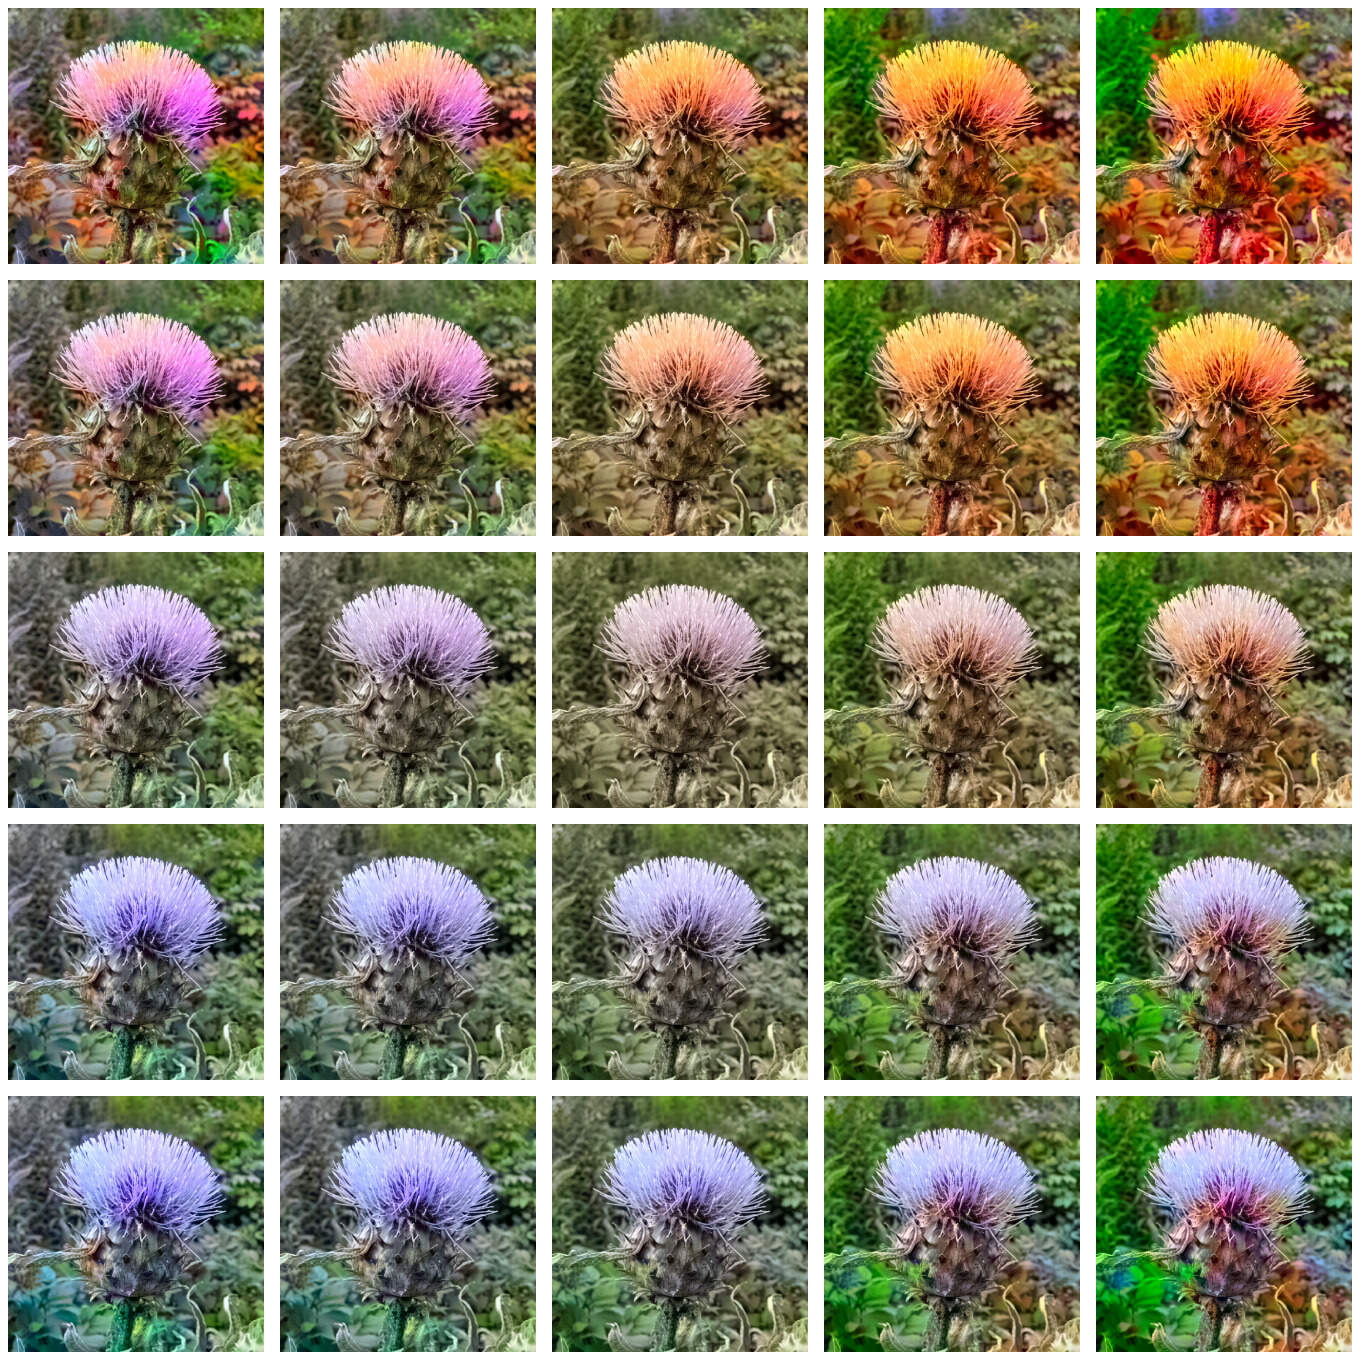} 
\end{figure}

\begin{figure*}
\centering
\includegraphics[width=1.0\textwidth]{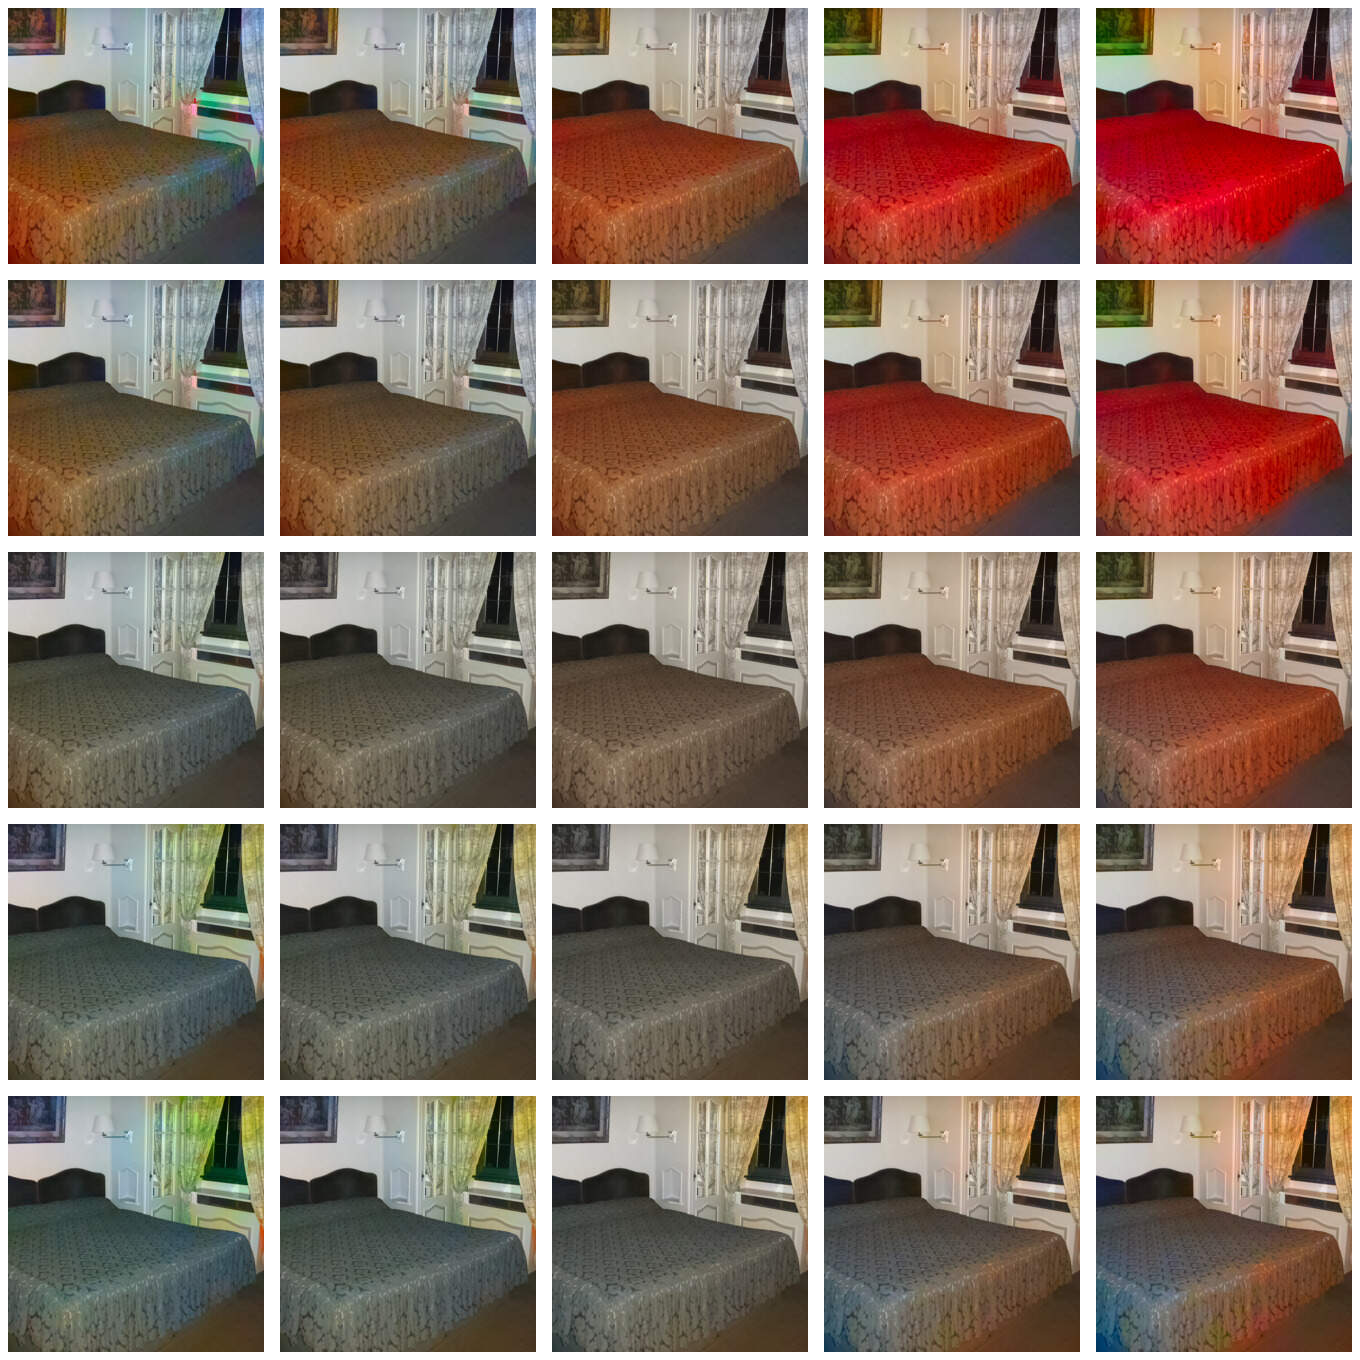} 
\end{figure*}

\FloatBarrier
%   
%   % TODO not in overleaf, because too big
%   \subsection{Colorization -- Additional examples}
%   \noindent
%   On the following pages, we provide some additional colorized images, as well as comparisons to alternative methods.
%   All images are taken from the ImageNet 2012 validation set, and all methods were trained on ImageNet 2012.
%   As we do not observe any significant diversity for the cGAN, we only provide a single sample.
%   
%   \subsubsection{General examples}
%   
%   \subsubsection{Humans}
%   \noindent
%   We find that the cINN often has difficulties generating convincing skin colors, as shown below.
%   Clothing is colored in diverse ways, but not always with the correct connectivity and consistency.
%   
%   \subsubsection{Lacking consistency}
%   \noindent
%   The following failure cases exhibit a lack in consistency, in occluded objects, multi-part objects, or reflections.
%   
%   \subsubsection{Color ignores semantic content}
%   \noindent
%   In the following examples, the semantic content of the image was not recognized, and the generated colors are clearly incorrect.
%   
%   \subsubsection{Outright failures}
%   \noindent
%   For the following images, the cINN fails completely, and generates colors with seemingly little or no connection to the grayscale image.
