# Supplementary material for: Conditional Invertible Neural Networks for Diverse Image-to-Image Translation
Source: arXiv:2105.02104 source file (2021-05-05)
Supplement: Supplementary file 4 [file 05_appendix_mnist.tex]

\subsection{Class-conditional generation for MNIST}

\noindent
To examine the behaviour of the INN without the conditioning network, we perform class-conditional generation of MNIST digits.
We construct a INN of 24 CCBs using fully connected subnetworks $s$ and $t$, 
which receive the conditioning directly as a one-hot vector.

\begin{wrapfigure}{R}{0.5\linewidth}
        \includegraphics[width=\linewidth]{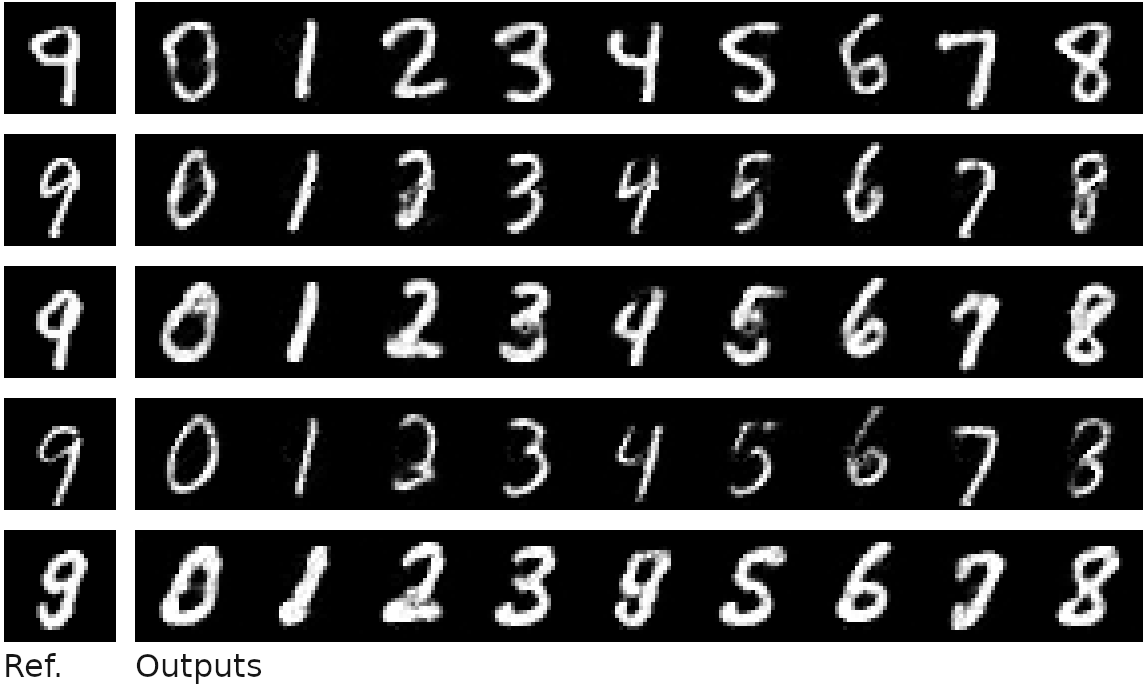}%
        \vspace{-2mm}
    	{\caption{To perform style transfer, we determine the latent code $\z = f(\x; \cond, \theta)$ of a test image \emph{(left)}, 
    	then use the inverse network $g = f^{-1}$ with different conditions ${\cond'}$ to generate the other digits in the same style, 
    	${\x'} = g(\z; {\cond'}, \theta)$.}
    	\label{fig:mnist_transfer}}
    \vspace{-3mm}
\end{wrapfigure}

Samples generated by the model are shown in \cref{fig:mnist_samples}. 
We find that the cINN learns latent representations that are shared across conditions $\cond$.
Keeping the latent vector $\z$ fixed while varying $\cond$ produces different digits in the same style.
This property, in conjunction with our network's invertibility, can directly be used for style transfer, as demonstrated in \cref{fig:mnist_transfer}.
This outcome is not obvious -- the trained cINN could also decompose into 10 essentially separate subnetworks, one for each condition.
In this case, the latent space of each class would be structured differently, and inter-class transfer of latent vectors would be meaningless.
The structure of the latent space is further illustrated in \cref{fig:mnist_attributes}, where we identify three latent axes with interpretable meanings.
Note that while the latent space is learned without supervision, we found the axes in a semi-automatic fashion:
We perform PCA on the latent vectors of the test set, without the noise augmentation, and manually identify meaningful directions in the subspace of the first four principal components.
\begin{figure}
\begin{center}
    \parbox{0.73\linewidth}{
    	{  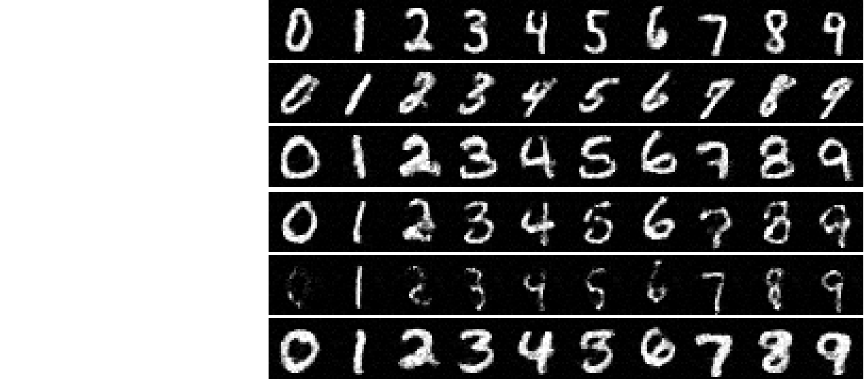 }
    	\vspace{-6mm}
    	{\caption{MNIST samples from our cINN conditioned on digit labels.
    	All ten digits within one row $(0, \dotsc, 9)$ were generated using the same latent code $\z$, but changing condition $\cond$.
    	We see that each $\z$ encodes a single style consistently across digits, while varying $\z$ between rows leads to strong differences in writing style.% \CR{line x is fat, ...}
    	} \label{fig:mnist_samples}}}
\end{center}
\end{figure}

\begin{figure}
    \centering
    \includegraphics[width=1.0\textwidth]{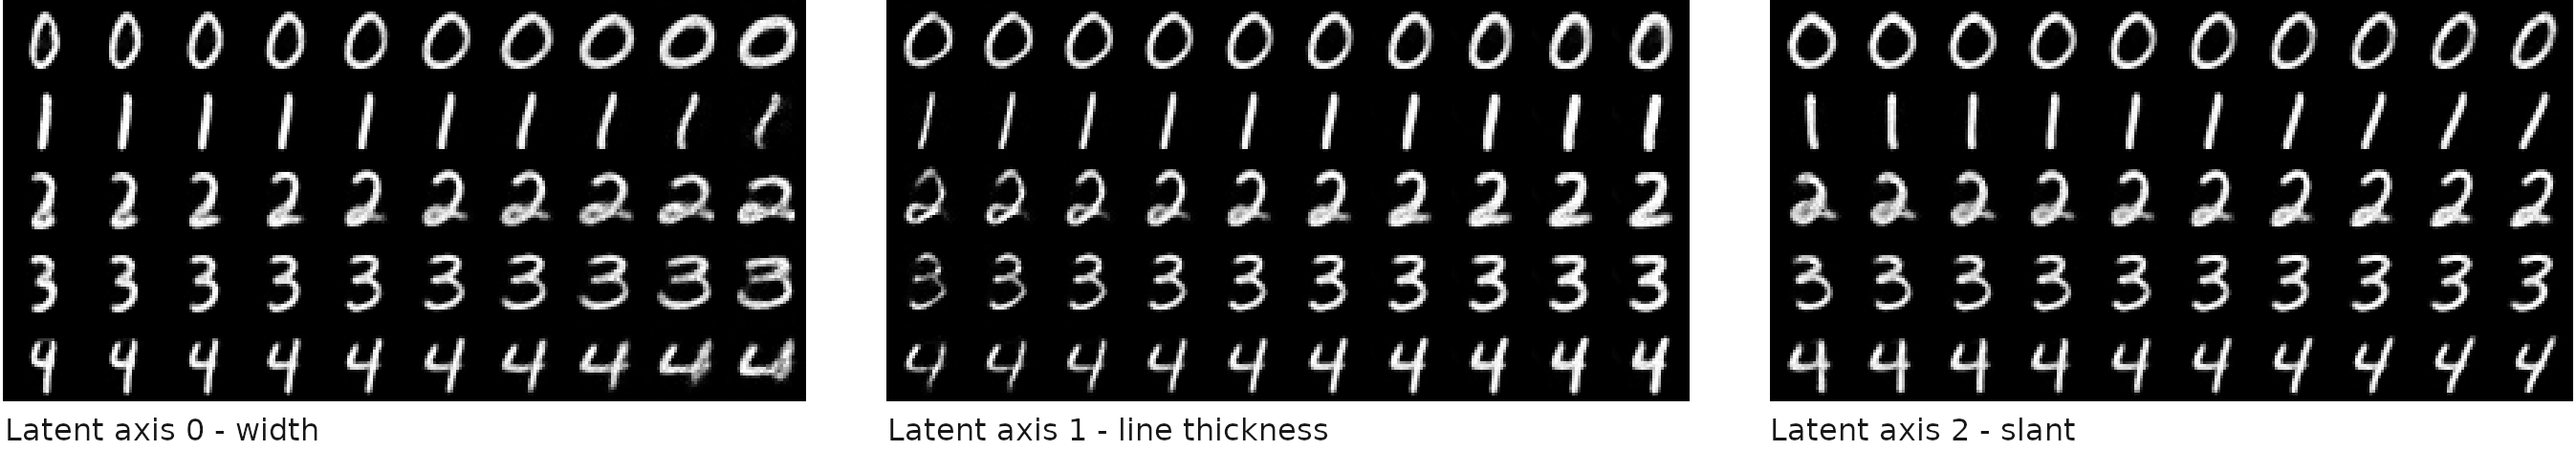}%
    \vspace{-4mm}%
	\caption{Axes in our MNIST model's latent space, which linearly encode the style attributes width, thickness and slant.}
	\vspace{-5mm}
	\label{fig:mnist_attributes}
\end{figure}
