# Supplementary material for: Conditional Invertible Neural Networks for Diverse Image-to-Image Translation
Source: arXiv:2105.02104 source file (2021-05-05)
Supplement: Supplementary file 5 [file 05_appendix_proofs.tex]

\section{Proofs and Assumptions}

\newcommand{\cn}{\varphi}
\newcommand{\Go}{\mathcal{G}_0}
\newcommand{\Gi}{\mathcal{G}_1}
\newcommand*{\QED}[1][$\square$]{%
\leavevmode\unskip\penalty9999 \hbox{}\nobreak\hfill
    \quad\hbox{#1}%
}

We further disambiguate the notation used in the main paper:
upper case letter (e.g. $X$) denote random variables (RVs),
and lower case letters denote their instances (e.g. $x$).
We write the probability distribution of a RV as $p(X)$,
and its evaluated density at any point $p(x)$, or $p(X=x)$ where ambiguous.
We include the INNs network parameters $\theta$ implicitly in $f$, and write
$f(\cdot; \hat \theta) \eqqcolon \hat f(\cdot)$, as well as
$q(x \mid c, \theta) \eqqcolon q(x \mid c)$ and 
$q(x \mid c, \hat \theta) \eqqcolon \hat q(x \mid c)$,
to simplify the equations.
We also write the loss as a functional depending on $f$ and $\cn$ for clarity:
$\cml = \cml[ f, \cn]$.
We also understand the argmin and argmax operations to return a set,
because the extremum must not necessarily be unique.
So, we write $\hat a \in \operatorname{arg\,min}\mathcal{L}(a)$ instead of `$=$' as in the main paper.
We also restate the propositions according to this notation.

We consider the RVs $X,Y$ jointly: $[X,Y] :\Omega \to (\mathcal{X}, \mu)$ 
with the measurable space $(\mathcal{X}, \mu)$ ,
where $\mathcal{X} = \mathcal{X}_X \times \mathcal{X}_Y = \mathbb{R}^{d_X + d_Y}$ 
is the domain of $x, y$,
and $\mu$ is the Lebesgue measure.
We assume $p(X,Y)$ is absolutely continuous w.r.t. $\mu$.
We make use of the differential entropy and differential conditional entropy $H$,
see \cite[Ch. 8.1]{cover2012elements} for definitions.

For the loss, we do not take a finite number of training samples into account,
and instead assume that the loss $\cml[f, \cn]$ is the exact expecation over the training data distribution $p(X,Y)$.
Strong consistency of the loss for the empirical expectation can be shown in the usual way,
assuming a compact parameter space and bounded outputs of the INN,
and applying Chebyshev's Inequality, but this is beyond the scope of this work,
and greatly complicates the form of the propositions.

To outline the proofs in the following section:
We first state and discuss some assumptions about the INN $f$ and the conditioning network $\cn$,
which are required in our proofs of the propositions.
Lemma 1 states two inequalities, which bound the loss from below.
Under Assumptions 1, 2 and 3, we show that choices of $f$ and $\cn$ exist 
where each bound is met exactly.
Lastly, for each proposition, we show that when the respective bound from Lemma 1 is met exactly,
the Proposition holds true.
\\[3mm]
\textbf{Assumption 1. }{\it
We assume that the INN is chosen from a family of distributional universal approximators $\mathcal{F}$,
as defined in \cite{teshima2020coupling}.
}
\\[3mm]
This simply means that the INN is in principle powerful enough to represent any distribution $p(X\mid C)$.
Affine coupling block INNs specifically were recently proven to satisfy this in \cite{teshima2020coupling},
under some requirements for the subnetworks.
Their result readily generalizes to CCBs, by changing the definition for $\mathcal{H}$ in Sec. D of \cite{teshima2020coupling}.
Proving this rigorously is beyond the scope of this work, 
so we leave the universality of the INN as an assumption.
\\[3mm]
\textbf{Assumption 2.}{\it
We assume that the conditioning network $\cn: \mathbb{R}^{d_Y} \to \mathbb{R}^{d_C}$
is chosen from the set $\Go$, which is defined as the set of all functions, 
for which the pushforward measure $p(C) \equiv p(\cn(Y)) \coloneqq \cn \sharp p(Y)$ is absolutely continuous w.r.t. the Lebesgue measure.
}
\\[3mm]
What this means intuitively, is that no subset of features can be exactly the same, 
or otherwise perfectly inter-dependent.
This is mostly a formal requirement: 
if it is not fulfilled, it does damage or alter the outcome of the training,
it simply means the MI is ill-defined, and Proposition 1 can not be formulated in the same way.
Proposition 2 can still be shown, by slightly altering Lemma 1 to avoid using the MI,
see e.g. \cite{beaudry2011intuitive} for an alternative formulation of the data processing inequality,
that applies even if the assumption does not hold.
\\[3mm]
\textbf{Assumption 3. }{\it
In addition to Assumption 2,
we assume that $\cn$ is chosen from $\Gi$, 
where $\Gi$ is a family of universal approximators as defined in \cite{hornik1989multilayer}.
Secondly, we assume the number of features extracted, $d_C \coloneqq \dim(C)$
is $\geq d_Y \coloneqq \dim(Y)$.
}\\[3mm]
This assumption is stronger than Assumption 2, and is a sufficient condition to show Proposition 2.
Intuitively, it says that $\cn$ must have sufficient expressive power so that the features $C$ 
can be informative enough for the INN to reproduce the true posterior.
This includes the number of features, and the network power.
If the features are too few, or inaccurate and uninformative, 
the INN will not be able to model the true posterior. \\[3mm]
\noindent
\textbf{Lemma 1. }{\it
Denoting the pushforward measure as $p(C) \equiv p(\cn(Y)) \coloneqq \cn \sharp p(Y)$,
the following inequality holds for all choices of $\cn$, $f$:
\begin{equation}
    \cml[f, \cn] 
    \underset{(a)}{\geq} H\big(X \mid \cn(Y)\big)
    \underset{(b)}{\geq} H\big(X \mid Y \big)
\end{equation}
Under Assumption 1, a choice of $f \in \mathcal{F}$ exists where (a) is equal, 
and under Assumption 3 a choice of $\cn \in \Gi$ exists where (b) becomes equal.
} \\[3mm] \noindent
\textbf{Proof. }{
    Because $\cml$ is equivalent to the definition of the differential cross-entropy $H_p(q(X\mid \cn(Y)))$,
    (a) follows directly from the inequality that the cross entropy is $\geq$ the entropy 
    with equality iff $p = q$ \cite[p. 256]{cover2012elements}.
    Assumption 1 guarantees that $f$ can be chosen so that $p(X\mid \cn(Y)) = q(X \mid \cn(Y))$,
    and therefore (a) becomes `='.

    (b) follows from the information processing inequality \cite[p. 34]{cover2012elements},
    whereby
    \begin{equation}
        I(X, Y) \geq I(X, \cn(Y)).
        \label{eq:data_processing}
    \end{equation}
    Writing out the terms, and subtracting the constant $H(X)$ from both sides directly yields (b).
    Therefore, (b) becomes `=' iff Eq. \ref{eq:data_processing} is also `='.
    We can construct a $\cn$ for which this is the case using Assumption 3 as a sufficient condition:
    We split up $C$ into $C = [C_s, C_n]$, where $\dim(C_s) = \dim(Y)$ and $\dim(C_n) = \dim(C) - \dim(Y) \geq 0$.
    According to \cite[Corollary 4.2]{hornik1989multilayer},
    we can choose $\cn$ such that that the mapping $\cn_s: Y \to C_s$ is a homeomorphism,
    and $C_n$ only contains constants (or noise), independent of $Y$. This part can effectively be ignored.
    Using this construction, we get
    \begin{equation}
        I(X, \cn(Y)) = I(X, \cn_s(Y)) = I(X, Y).
    \end{equation}
    We used the independence of $C_n$ and $Y$ in the first step, 
    and the invariance of the MI under homeomorphic transforms \cite[Eq. A2]{kraskov2004estimating}
    in the second step.
    \QED
}
\\[3mm]
\textbf{Proposition 1. }{\it
Let $\hat f$ be the INN and $\hat \cn$ the conditioning network that jointly minimize $\cml$,
where $\cn$ is optimized over $\Go$ given in Assumption 2, and $f$ over $\mathcal{F}$ given in Assumption 1.
Then it holds that
\begin{equation}
    I \big(X, \hat \cn(Y) \big) = \underset{\varphi \in \Go}{\operatorname {max}} \; I \big(X, \cn(Y) \big) 
\end{equation}
}
\\[3mm]
\textbf{Proof.}
Recall the minimization process
\begin{equation}
    \hat f, \hat \cn \in \underset{f, \cn \in \mathcal{F} \times \Go}{\operatorname{arg\,min}} \cml[f, \cn]
\end{equation}
By definition, we then have
\begin{equation}
    \cml[\hat f, \hat \cn] = \underset{\cn\in\Go}{\mathrm{min}} \cml[\hat f, \cn]
    \label{eq:loss_phi_max}
\end{equation}
Using Assumption 1, we have already shown that (a) in Lemma 1 will be `=' for $\hat f$ and arbitrary $\cn$, 
the loss has its minimum possible value w.r.t.~$f$, and the bound can be reached exactly.
We use the equality to substitute $\cml$ in Eq. \ref{eq:loss_phi_max}:
\begin{equation}
    H(X|\hat \cn(Y)) = \underset{\cn\in\Go}{\mathrm{min}} H(X| \cn(Y)) 
\end{equation}
As a final step, we subtract the constant $H(X)$ to both sides.
It can be written inside the $\mathrm{min}()$ operation, 
as it does not depend on $\cn$.
Writing out the entropies and rearranging the terms directly gives
\begin{equation}
    - I(X, \hat \cn(Y)) = \underset{\cn\in\Go}{\mathrm{min}} - I(X, \cn(Y)) 
\end{equation}
\QED
\\[3mm]
\textbf{Proposition 2. }{\it
Assume $\cn$ is optimized over $\Gi$ and $\dim(C) \geq \dim(Y)$ (Assumption 3),
and $f$ is optimized over $\mathcal{F}$ (Assumption 1).
Then the following holds for $\hat f, \hat \cn \in \operatorname{arg\,min}{\cml[f, \cn]}$:
\begin{equation}
    \hat q(X | \hat \cn(Y)) = p(X|Y)
\end{equation}
}
\\[3mm]
\textbf{Proof.}
We consider the KL-divergence between the true and learned posterior,
write it out, and identify the loss and the conditional entropy:
\begin{align}
    D_\mathrm{KL}\big( p(X\mid Y) \| \hat q(X \mid \hat \cn(Y))\big) \\
    = \cml[f, \cn] - H(X\mid Y)
\end{align}
In Lemma 1, we showed that $H(X\mid Y)$ is the global minimum of the loss,
and will be reached in training under Assumptions 1, 2, and 3 ((a) and (b) both `=').
Then we can immediately see that the KL-divergence is zero, 
which is the case iff the two distributions are identical.
\QED
